# Supplementary material for: A new threshold reveals the uncertainty about the effect of school opening on diffusion of Covid-19
Source: arXiv:2104.04136 source file (2021-04-12)
Supplement: Supplementary file 1 [file MathStudySchoolOpening-OnlineMaterial-CriticalBounds.pdf]

# Critical bounds

## Outbreak - Sections 2.1, 4.6

In[∘]:=
```
BB = { {beta11 S10 - 1, beta12 S10}, {beta21 S20, beta22 S20 - 1}}
```

Out[∘]=
```
{{-1 + beta11 S10, beta12 S10}, {beta21 S20, -1 + beta22 S20}}
```

In[∘]:=
```
MatrixExp[BB t];
```

In[∘]:=
```
II = MatrixExp[BB t].{I10, I20};
```

### Critical point

In[∘]:=
```
beta22 S20 / S10 /. {beta22 → 2, S10 → 0.2, S20 → 0.8 - 0.00003}
```

Out[∘]=
```
7.9997
```

### Bound with epsilon = eps =0.3

In[∘]:=
```
Solve[{I1tau - I10 == (beta11 S10 - 1) JJI + beta12 S10 HHI,
   I2tau - I20 == beta21 S20 JJI + (beta22 S20  - 1) HHI}, {JJI, HHI}]
```

Out[∘]=

$$\left\{\left\{JJI \to -\frac{I10 - I1tau + beta12\ I20\ S10 - beta12\ I2tau\ S10 - beta22\ I10\ S20 + beta22\ I1tau\ S20}{-1 + beta11\ S10 + beta22\ S20 + beta12\ beta21\ S10\ S20 - beta11\ beta22\ S10\ S20},\right.\right.$$
$$\left.\left. HHI \to -\frac{I20 - I2tau - beta11\ I20\ S10 + beta11\ I2tau\ S10 + beta21\ I10\ S20 - beta21\ I1tau\ S20}{-1 + beta11\ S10 + beta22\ S20 + beta12\ beta21\ S10\ S20 - beta11\ beta22\ S10\ S20}\right\}\right\}$$

In[∘]:=
```
DeltaS1 = I1tau - I10 + JJI /. {JJI →
      - ((I10 - I1tau + beta12 I20 S10 - beta12 I2tau S10 - beta22 I10 S20 + beta22 I1tau S20) /
          (-1 + beta11 S10 + beta22 S20 + beta12 beta21 S10 S20 - beta11 beta22 S10 S20)), HHI →
      - ((I20 - I2tau - beta11 I20 S10 + beta11 I2tau S10 + beta21 I10 S20 - beta21 I1tau S20) /
          (-1 + beta11 S10 + beta22 S20 + beta12 beta21 S10 S20 - beta11 beta22 S10 S20))};
DeltaS1 = DeltaS1 /. {I1tau → II[[1]],
     I2tau → II[[2]]};
DeltaS2 = I2tau - I20 + HHI /. {JJI →
      - ((I10 - I1tau + beta12 I20 S10 - beta12 I2tau S10 - beta22 I10 S20 + beta22 I1tau S20) /
          (-1 + beta11 S10 + beta22 S20 + beta12 beta21 S10 S20 - beta11 beta22 S10 S20)), HHI →
      - ((I20 - I2tau - beta11 I20 S10 + beta11 I2tau S10 + beta21 I10 S20 - beta21 I1tau S20) /
          (-1 + beta11 S10 + beta22 S20 + beta12 beta21 S10 S20 - beta11 beta22 S10 S20))};
DeltaS2 = DeltaS2 /. {I1tau → II[[1]],
     I2tau → II[[2]]};
```

In[∘]:=
```
DeltaS = (DeltaS1 + DeltaS2);
```

In[∘]:=
```
DeltaS = Simplify[DeltaS];
```

In[∘]:=
```
DeltaS5 = DeltaS /. t → 5;
```

In[∘]:=
```
DeltaS50 = DeltaS5 /. beta11 → 0;
```

In[∘]:=
```
Inc = DeltaS5 / DeltaS50 /. {beta22 → 2, beta12 → 0.5, beta21 → 0.5,
     I10 → 0, S10 → 0.2, I20 → 0.00003, S20 → 0.8 - 0.00003};
```

In[•]:=
```
Plot[Inc, {beta11, 0, 8}]
```

Out[•]=
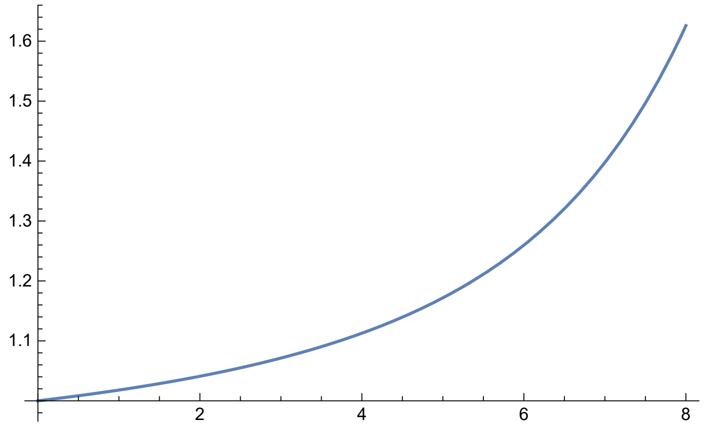


In[•]:=
```
FindRoot[Inc == 1.3, {beta11, 1}]
```

Out[•]=
```
{beta11 → 6.34431}
```

**Lack of singularity at the value of beta11 that makes the denominator zero is not**

In[•]:=
```
Clear[II]
```

In[•]:=
```
Solve[{I1tau - I10 == (beta11 S10 - 1) JJI + beta12 S10 HHI,
   I2tau - I20 == beta21 S20 JJI + (beta22 S20 - 1) HHI}, {JJI, HHI}]
```

Out[•]=
$$\left\{\left\{JJI \to -\frac{I10 - I1tau + beta12\ I20\ S10 - beta12\ I2tau\ S10 - beta22\ I10\ S20 + beta22\ I1tau\ S20}{-1 + beta11\ S10 + beta22\ S20 + beta12\ beta21\ S10\ S20 - beta11\ beta22\ S10\ S20},\ HHI \to -\frac{I20 - I2tau - beta11\ I20\ S10 + beta11\ I2tau\ S10 + beta21\ I10\ S20 - beta21\ I1tau\ S20}{-1 + beta11\ S10 + beta22\ S20 + beta12\ beta21\ S10\ S20 - beta11\ beta22\ S10\ S20}\right\}\right\}$$

In[•]:=
```
DeltaS1 = I1tau - I10 + JJI /. {JJI →
     - ((I10 - I1tau + beta12 I20 S10 - beta12 I2tau S10 - beta22 I10 S20 + beta22 I1tau S20) /
        (-1 + beta11 S10 + beta22 S20 + beta12 beta21 S10 S20 - beta11 beta22 S10 S20)), HHI →
     - ((I20 - I2tau - beta11 I20 S10 + beta11 I2tau S10 + beta21 I10 S20 - beta21 I1tau S20) /
        (-1 + beta11 S10 + beta22 S20 + beta12 beta21 S10 S20 - beta11 beta22 S10 S20))};
DeltaS2 = I2tau - I20 + HHI /. {JJI → - ((I10 - I1tau + beta12 I20 S10 -
          beta12 I2tau S10 - beta22 I10 S20 + beta22 I1tau S20) /
        (-1 + beta11 S10 + beta22 S20 + beta12 beta21 S10 S20 - beta11 beta22 S10 S20)), HHI →
     - ((I20 - I2tau - beta11 I20 S10 + beta11 I2tau S10 + beta21 I10 S20 - beta21 I1tau S20) /
        (-1 + beta11 S10 + beta22 S20 + beta12 beta21 S10 S20 - beta11 beta22 S10 S20))};
```

In[•]:=
```
DeltaS = (DeltaS1 + DeltaS2);
```

In[•]:=
```
DeltaS = Simplify[DeltaS]
```

Out[•]=
```
((beta21 (I10 - I1tau) + beta22 (I20 - I2tau)) S20 +
    beta12 S10 (I20 + beta21 (I10 - I1tau) S20 + beta21 I20 S20 - I2tau (1 + beta21 S20)) +
    beta11 S10 (I10 - beta22 I10 S20 + beta22 (-I20 + I2tau) S20 + I1tau (-1 + beta22 S20))) /
  (1 - beta22 S20 - beta12 beta21 S10 S20 + beta11 S10 (-1 + beta22 S20))
```

In[•]:=
```
Solve[-1 + beta11 S10 + beta22 S20 + beta12 beta21 S10 S20 - beta11 beta22 S10 S20 == 0, beta11]
```

Out[•]=
$$\left\{\left\{beta11 \to \frac{-1 + beta22\ S20 + beta12\ beta21\ S10\ S20}{S10\ (-1 + beta22\ S20)}\right\}\right\}$$

In[•]:=
```
DeltaSt = (DeltaS1 + DeltaS2) /. {beta22 → 2, beta12 → 0.5, beta21 → 0.5,
     tau → 2, n1 -> 0.2, n2 → 0.8, I10 → 0, S10 → 0.2, I20 → 0.00003, S20 → 0.8 - 0.00003};
```

The next value is to be compared to 8, illustrating the difference between the critical point and the zero of the denominator:

In[∘]:=
```
(-1 + beta22 S20 + beta12 beta21 S10 S20)/(S10 (-1 + beta22 S20)) /. {beta22 → 2, beta12 → 0.5, beta21 → 0.5,
  tau → 2, n1 -> 0.2, n2 → 0.8, I10 → 0, S10 → 0.2, I20 → 0.00003, S20 → 0.8 - 0.00003}
```

Out[∘]= 5.33335

We take the value of the DeltaS at the beta11 that makes the denominator zero to show that it is not divergent:

In[∘]:=
```
DeltaSt = DeltaSt /. {I1tau → II[[1]],
    I2tau → II[[2]]};
```

In[∘]:=
```
DeltaSt =
 DeltaSt /. {beta11 → 5.333354168750209`, beta22 → 2, beta12 → 0.5, beta21 → 0.5,
   tau → 2, n1 -> 0.2, n2 → 0.8, I10 → 0, S10 → 0.2, I20 → 0.00003, S20 → 0.8 - 0.00003}
```

Out[∘]=
$$-0.00003 + 0.00003 \left(-0.150013\, e^{1.66533\times10^{-16}\, t} + 0.150013\, e^{0.666611\, t}\right) + 0.00003 \left(0.100015\, e^{1.66533\times10^{-16}\, t} + 0.899985\, e^{0.666611\, t}\right) + 9.0072\times10^{15} \left(3.\times10^{-6} + 0.0000179982 \left(-0.150013\, e^{1.66533\times10^{-16}\, t} + 0.150013\, e^{0.666611\, t}\right) - 3.\times10^{-6} \left(0.100015\, e^{1.66533\times10^{-16}\, t} + 0.899985\, e^{0.666611\, t}\right)\right) + 9.0072\times10^{15} \left(-2.00013\times10^{-6} - 0.0000119996 \left(-0.150013\, e^{1.66533\times10^{-16}\, t} + 0.150013\, e^{0.666611\, t}\right) + 2.00013\times10^{-6} \left(0.100015\, e^{1.66533\times10^{-16}\, t} + 0.899985\, e^{0.666611\, t}\right)\right)$$

In[∘]:=
```
Plot[DeltaSt, {t, -8, 8}]
```

Out[∘]=
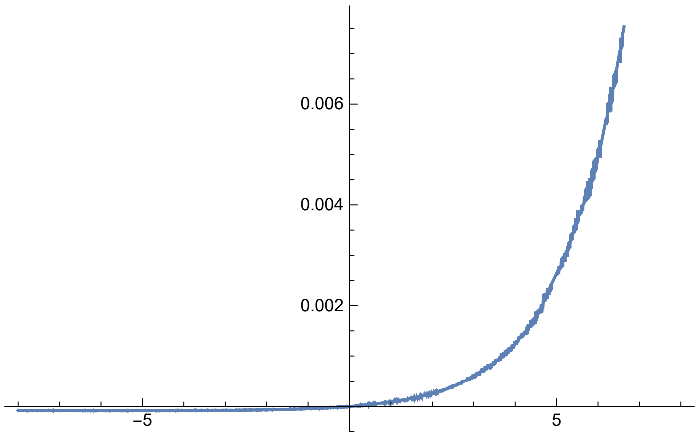


The above values are finite, hence not diverging.

## Lockdown - Sections 2.2, 4.8

### Critical point

In[∘]:=
```
Solve[{-I1tau == (beta11 S1tau - 1) JJLI + beta12 S1tau HHLI,
   -I2tau == beta21 S2tau JJLI + (beta22 S2tau - 1) HHLI}, {JJLI, HHLI}]
```

Out[∘]=

$$\left\{\left\{JJLI \to -\frac{I1tau + beta12\ I2tau\ S1tau - beta22\ I1tau\ S2tau}{-1 + beta11\ S1tau + beta22\ S2tau + beta12\ beta21\ S1tau\ S2tau - beta11\ beta22\ S1tau\ S2tau},\ HHLI \to -\frac{I2tau - beta11\ I2tau\ S1tau + beta21\ I1tau\ S2tau}{-1 + beta11\ S1tau + beta22\ S2tau + beta12\ beta21\ S1tau\ S2tau - beta11\ beta22\ S1tau\ S2tau}\right\}\right\}$$

In[∘]:=

$$DeltaSL1 = -I1tau + JJLI\ /.\ \left\{JJLI \to -\frac{I1tau + beta12\ I2tau\ S1tau - beta22\ I1tau\ S2tau}{-1 + beta11\ S1tau + beta22\ S2tau + beta12\ beta21\ S1tau\ S2tau - beta11\ beta22\ S1tau\ S2tau},\ HHLI \to -\frac{I2tau - beta11\ I2tau\ S1tau + beta21\ I1tau\ S2tau}{-1 + beta11\ S1tau + beta22\ S2tau + beta12\ beta21\ S1tau\ S2tau - beta11\ beta22\ S1tau\ S2tau}\right\}$$

$$DeltaSL2 = -I2tau + HHLI\ /.\ \left\{JJLI \to -\frac{I1tau + beta12\ I2tau\ S1tau - beta22\ I1tau\ S2tau}{-1 + beta11\ S1tau + beta22\ S2tau + beta12\ beta21\ S1tau\ S2tau - beta11\ beta22\ S1tau\ S2tau},\ HHLI \to -\frac{I2tau - beta11\ I2tau\ S1tau + beta21\ I1tau\ S2tau}{-1 + beta11\ S1tau + beta22\ S2tau + beta12\ beta21\ S1tau\ S2tau - beta11\ beta22\ S1tau\ S2tau}\right\}$$

In[∘]:=
```
DeltaSL = Simplify[DeltaSL1 + DeltaSL2]
```

Out[∘]=
```
((beta21 I1tau + beta22 I2tau) S2tau +
    beta12 S1tau (I2tau + beta21 I1tau S2tau + beta21 I2tau S2tau) -
    beta11 S1tau (beta22 I2tau S2tau + I1tau (-1 + beta22 S2tau))) /
  (1 - beta22 S2tau - beta12 beta21 S1tau S2tau + beta11 S1tau (-1 + beta22 S2tau))
```

Singularity of denominator:

In[∘]:=
```
Solve[
 1 - beta22 S2tau - beta12 beta21 S1tau S2tau + beta11 S1tau (-1 + beta22 S2tau) == 0, beta11]
```

Out[∘]=

$$\left\{\left\{beta11 \to \frac{-1 + beta22\ S2tau + beta12\ beta21\ S1tau\ S2tau}{S1tau\ (-1 + beta22\ S2tau)}\right\}\right\}$$

Numerator does not vanish at the zero of the denominator:

In[∘]:=

$$Simplify\Big[((beta21\ I1tau + beta22\ I2tau)\ S2tau + beta12\ S1tau\ (I2tau + beta21\ I1tau\ S2tau + beta21\ I2tau\ S2tau) - beta11\ S1tau\ (beta22\ I2tau\ S2tau + I1tau\ (-1 + beta22\ S2tau)))\ /.\ \left\{beta11 \to \frac{-1 + beta22\ S2tau + beta12\ beta21\ S1tau\ S2tau}{S1tau\ (-1 + beta22\ S2tau)}\right\}\Big]$$

Out[∘]=

$$\frac{(1 + beta21\ S2tau - beta22\ S2tau)\ (-beta12\ I2tau\ S1tau + I1tau\ (-1 + beta22\ S2tau))}{-1 + beta22\ S2tau}$$

In[∘]:=
```
(1 + beta21 S2tau - beta22 S2tau) (-beta12 I2tau S1tau + I1tau (-1 + beta22 S2tau)) /.
 {beta22 → 1, beta12 → 0.25, beta21 → 0.25,
  S2tau → 0.7, S1tau → 0.15,
  I1tau → 0.0001, I2tau → 0.0001}
```
Out[∘]= -0.0000160313

**Numerical evaluation of critical point**

In[∘]:=
```
1 / S1tau - (beta12 beta21 S2tau) / (1 - beta22 S2tau) /.
 {beta22 → 1, beta12 → 0.25, beta21 → 0.25,
  S2tau → 0.7, S1tau → 0.15,
  I1tau → 0.0001, I2tau → 0.0001}
```
Out[∘]= 6.52083

**Bound with epsilon = eps**

In[∘]:=
```
Solve[(beta11 (I2tau S1tau) - I1tau - I2tau -
      beta12 I2tau S1tau - beta21 I1tau S2tau + beta22 I1tau S2tau) /
    (beta11 S1tau (1 - beta22 S2tau) - 1 + beta22 S2tau + beta12 beta21 S1tau S2tau) ==
   ((-I1tau - I2tau - beta12 I2tau S1tau - beta21 I1tau S2tau + beta22 I1tau S2tau) /
     (-1 + beta22 S2tau + beta12 beta21 S1tau S2tau)) (1 + eps), beta11];
```

In[∘]:=
```
(eps (I1tau + I2tau + beta12 I2tau S1tau + beta21 I1tau S2tau - beta22 I1tau S2tau)
    (-1 + beta22 S2tau + beta12 beta21 S1tau S2tau)) /
  (S1tau (-I1tau - eps I1tau - eps I2tau - beta12 I2tau S1tau -
      beta12 eps I2tau S1tau - beta21 I1tau S2tau + 2 beta22 I1tau S2tau -
      beta21 eps I1tau S2tau + 2 beta22 eps I1tau S2tau + beta22 eps I2tau S2tau -
      beta12 beta21 I2tau S1tau S2tau + beta12 beta22 I2tau S1tau S2tau +
      beta12 beta22 eps I2tau S1tau S2tau + beta21 beta22 I1tau S2tau^2 -
      beta22^2 I1tau S2tau^2 + beta21 beta22 eps I1tau S2tau^2 - beta22^2 eps I1tau S2tau^2)) /.
 {beta22 → 1, beta12 → 0.25, beta21 → 0.25,
  S2tau → 0.798064, S1tau → 0.199622,
  I1tau → 1.601 × 10^{-4}, I2tau → 7.95554 × 10^{-4}}
```
Out[∘]= $\left\{-\frac{0.000865089\ \text{eps}}{-0.0000289176 - 0.000181647\ \text{eps}}\right\}$

**beta11 for epsilon = eps =0.3**

In[∘]:=
```
-(0.00029588281250000001` eps) / (-0.000016031250000000007` - 0.00004537499999999998` eps) /. eps → 0.3;
```

## Vaccinations - Sections 2.3, 4.14

**Formula (28) and (29)**

In[∘]:=
```
Itilde2 = Sum[(I20 + (β21 I10 S20)/(1 - β11 S10 + v i))
    Product[(β22 S20 + (β12 β21 S10 S20)/(1 - β11 S10 + r v)) / (1 + r v), {r, 1, i - 1}], {i, 1, Infinity}];
Itilde1 = (β12 * S10 * Itilde2 + I10) / (1 - β11 * S10);
```

**Formula (30)**

For the initial conditions S10, I10, S20, I20, see the Section entitled "Phase transition over vaccina-

tion phase" in the main file

```
In[]:= ΔI = -I10 - I20 + Itilde1 + Itilde2;
ΔIval = ΔI /. {β22 → 2, β12 → 0.5, β21 → 0.5, I10 → 1.97281×10^{-5},
    S10 → 0.198872, I20 → 9.55298×10^{-5}, S20 → 0.794451, v → 0.1};
ΔI0 = ΔIval /. {β11 → 0};

In[]:= Ratio = ΔIval / ΔI0;

In[]:= Plot[Ratio, {β11, 0, 5.5}, PlotRange → {1, 4}]
```

Out[]=

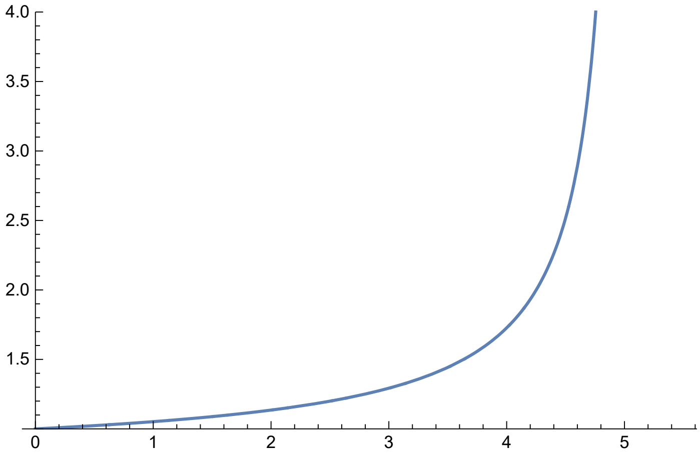


**beta11 for epsilon = eps = 0.3**

```
In[]:= FindRoot[Ratio - 1.3, {β11, 2}]

Out[]= {β11 → 3.03111}
```
