# Supplementary material for: A new threshold reveals the uncertainty about the effect of school opening on diffusion of Covid-19
Source: arXiv:2104.04136 source file (2021-04-12)
Supplement: Supplementary file 2 [file MathStudySchoolOpening-OnlineMaterial-Simulations.pdf]

This Mathematica File contains the simulations of the phase transition phenomenon in three different periods during the pandemic : 1. Outbreak Phase 2. Lockdown Phase 3. Vaccination Phase. Moreover, we include a joint plot of three phases together to illustrate the effect of different level of protective measures on the pandemic. In the last section, we include a graph illustrating the relation between the largest eigenvalues of a transmission matrix and its entries.

---

# OUTBREAK PHASE

## Phase transition over lockdown period

In[310]:=
```
T1 = 5;
T2 = 13;
gg = 1;
ss10 = 0.2;
ii10 = 0;
ss20 = .79997;
ii20 = .00003;
T = 15;
bb11 = 8.5;
bb22 = 2;
bb12 = 0.5;
bb21 = bb12;
SSS = NDSolve[{SS1'[t] == -bb11 SS1[t] × II1[t] - bb12 SS1[t] × II2[t],
    II1'[t] == bb11 SS1[t] × II1[t] + bb12 SS1[t] × II2[t] - gg II1[t],
    SS2'[t] == -bb21 SS2[t] × II1[t] - bb22 SS2[t] × II2[t],
    II2'[t] == bb21 SS2[t] × II1[t] + bb22 SS2[t] × II2[t] - gg II2[t],
    SS1[0] == ss10, II1[0] == ii10, SS2[0] == ss20, II2[0] == ii20},
   {SS1[t], II1[t], SS2[t], II2[t]}, {t, 0, T}, Method → "ExplicitRungeKutta"];
bb11 = 6.3;
SSSL = NDSolve[{SS1'[t] == -bb11 SS1[t] × II1[t] - bb12 SS1[t] × II2[t],
    II1'[t] == bb11 SS1[t] × II1[t] + bb12 SS1[t] × II2[t] - gg II1[t],
    SS2'[t] == -bb21 SS2[t] × II1[t] - bb22 SS2[t] × II2[t],
    II2'[t] == bb21 SS2[t] × II1[t] + bb22 SS2[t] × II2[t] - gg II2[t],
    SS1[0] == ss10, II1[0] == ii10, SS2[0] == ss20, II2[0] == ii20},
   {SS1[t], II1[t], SS2[t], II2[t]}, {t, 0, T}, Method → "ExplicitRungeKutta"];
bb11 = 0;
SSSC = NDSolve[{SS1'[t] == -bb11 SS1[t] × II1[t] - bb12 SS1[t] × II2[t],
    II1'[t] == bb11 SS1[t] × II1[t] + bb12 SS1[t] × II2[t] - gg II1[t],
    SS2'[t] == -bb21 SS2[t] × II1[t] - bb22 SS2[t] × II2[t],
    II2'[t] == bb21 SS2[t] × II1[t] + bb22 SS2[t] × II2[t] - gg II2[t],
    SS1[0] == ss10, II1[0] == ii10, SS2[0] == ss20, II2[0] == ii20},
   {SS1[t], II1[t], SS2[t], II2[t]}, {t, 0, T}, Method → "ExplicitRungeKutta"];
fig1 = Plot[{SSSC[[1, 4, 2]] + SSSC[[1, 2, 2]],
    SSSL[[1, 4, 2]] + SSSL[[1, 2, 2]], SSS[[1, 4, 2]] + SSS[[1, 2, 2]]},
   {t, 0, T1}, PlotLabels → {Style["β11=0", FontSize → 20],
     Style["β11=6.3", FontSize → 20], Style["β11=8.5", FontSize → 20]},
   PlotRange → Automatic, PlotStyle → {Cyan, Green, Red},
   AxesLabel → {Style["t", FontSize → 20], Style["I(t)", FontSize → 20]},
   TicksStyle → Directive[Black, 20]];

Plot[{SSSC[[1, 4, 2]] + SSSC[[1, 2, 2]],
  SSSL[[1, 4, 2]] + SSSL[[1, 2, 2]], SSS[[1, 4, 2]] + SSS[[1, 2, 2]]},
 {t, 0, T1}, PlotLabels → {Style["β11=0", FontSize → 20],
   Style["β11=6.3", FontSize → 20], Style["β11=8.5", FontSize → 20]},
 PlotRange → Automatic, PlotStyle → {Cyan, Green, Red},
 PlotLegends → Placed[{Style["Schools Closed", FontSize → 12],
    Style["Open Schools with Suitable Measures", FontSize → 12],
    Style["School Transmission Exceeding the Critical Value", FontSize → 12]}, Center],
 AxesLabel → {Style["t", FontSize → 20], Style["I(t)", FontSize → 20]},
 TicksStyle → Directive[Black, 20], ImageSize → Large]
```

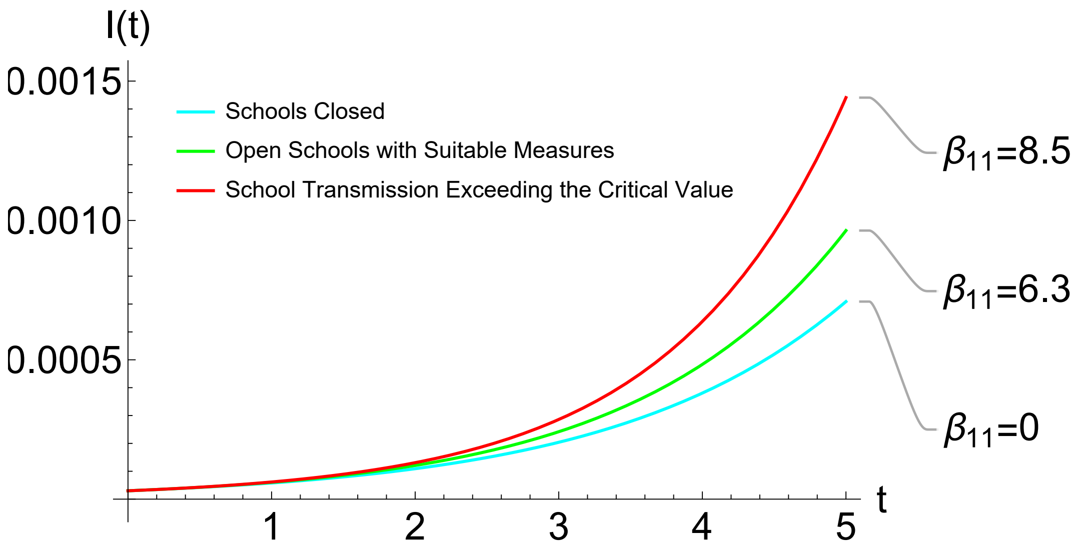
I(t)
0.0015
0.0010
0.0005
Schools Closed
Open Schools with Suitable Measures
School Transmission Exceeding the Critical Value
$\beta_{11}$=8.5
$\beta_{11}$=6.3
$\beta_{11}$=0
1
2
3
4
5
t

# LOCKDOWN PHASE

## Lockdown phase with school closed

In[330]:=
```
gg = 1;
T = 40;
ss10 = SSSC[[1, 1, 2]] /. t → T1;
ii10 = SSSC[[1, 2, 2]] /. t → T1;
ss20 = SSSC[[1, 3, 2]] /. t → T1;
ii20 = SSSC[[1, 4, 2]] /. t → T1;
bb11 = 0;
bb22 = 1;
bb12 = 0.25;
bb21 = bb12;
v = 0.1;
SSS0 = NDSolve[{
    SS1'[t] == -bb11 SS1[t] × II1[t] - bb12 SS1[t] × II2[t],
    II1'[t] == bb11 SS1[t] × II1[t] + bb12 SS1[t] × II2[t] - gg II1[t],
    SS2'[t] == -bb21 SS2[t] × II1[t] - bb22 SS2[t] × II2[t],
    II2'[t] == bb21 SS2[t] × II1[t] + bb22 SS2[t] × II2[t] - gg II2[t],
    SS1[0] == ss10, II1[0] == ii10, SS2[0] == ss20, II2[0] == ii20},
   {SS1[t], II1[t], SS2[t], II2[t]}, {t, 0, T}, Method → "ExplicitRungeKutta"];
fig2 = Plot[{SSS0[[1, 4, 2]] + SSS0[[1, 2, 2]]}, {t, 0, T2}, PlotLabels →
   {Style[ToString[Subscript[OverBar["β"], 11], FormatType → StandardForm] <> "=0",
     FontSize → 20]}, TicksStyle → Directive[Black, 20],
  PlotRange → Automatic, PlotStyle → Cyan, ImageSize → Large]
```

Out[342]=

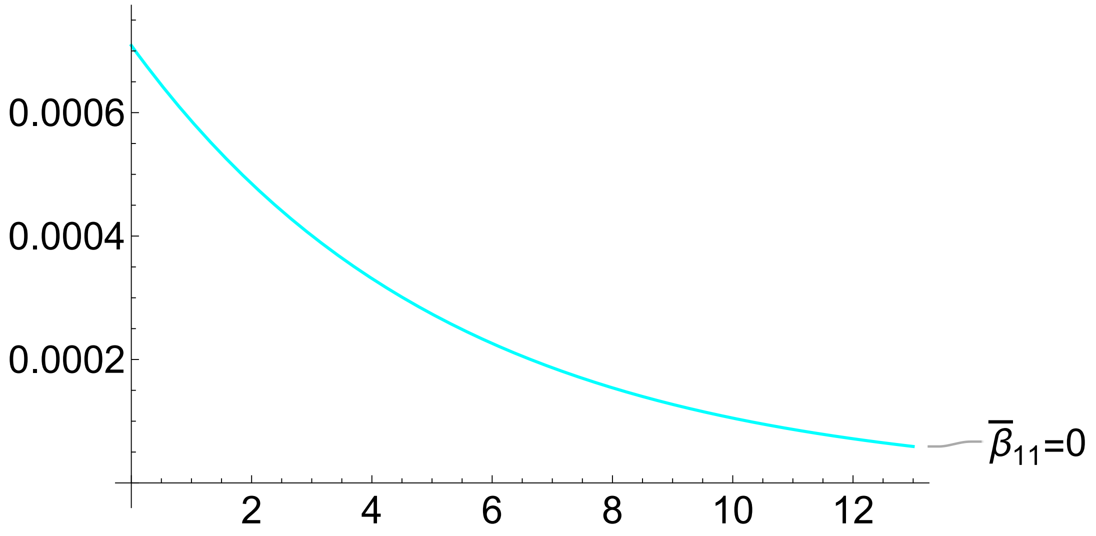

## Phase transition over lockdown phase

In[343]:=
```
gg = 1;
T = 40;
ss10 = SSSL[[1, 1, 2]] /. t → T1;
ii10 = SSSL[[1, 2, 2]] /. t → T1;
ss20 = SSSL[[1, 3, 2]] /. t → T1;
ii20 = SSSL[[1, 4, 2]] /. t → T1;
bb22 = 1;
bb12 = 0.25;
bb21 = bb12;
v = 0.1;
bb11 = 2.99;
SSS3 = NDSolve[{
    SS1'[t] == -bb11 SS1[t] × II1[t] - bb12 SS1[t] × II2[t],
    II1'[t] == bb11 SS1[t] × II1[t] + bb12 SS1[t] × II2[t] - gg II1[t],
    SS2'[t] == -bb21 SS2[t] × II1[t] - bb22 SS2[t] × II2[t],
    II2'[t] == bb21 SS2[t] × II1[t] + bb22 SS2[t] × II2[t] - gg II2[t],
    SS1[0] == ss10, II1[0] == ii10, SS2[0] == ss20, II2[0] == ii20},
   {SS1[t], II1[t], SS2[t], II2[t]}, {t, 0, T}, Method → "ExplicitRungeKutta"];

bb11 = 5;
SSS5 = NDSolve[{
    SS1'[t] == -bb11 SS1[t] × II1[t] - bb12 SS1[t] × II2[t],
    II1'[t] == bb11 SS1[t] × II1[t] + bb12 SS1[t] × II2[t] - gg II1[t],
    SS2'[t] == -bb21 SS2[t] × II1[t] - bb22 SS2[t] × II2[t],
    II2'[t] == bb21 SS2[t] × II1[t] + bb22 SS2[t] × II2[t] - gg II2[t],
    SS1[0] == ss10, II1[0] == ii10, SS2[0] == ss20, II2[0] == ii20},
   {SS1[t], II1[t], SS2[t], II2[t]}, {t, 0, T}, Method → "ExplicitRungeKutta"];


fig22 = Plot[{
   SSS3[[1, 4, 2]] + SSS3[[1, 2, 2]],
   SSS5[[1, 4, 2]] + SSS5[[1, 2, 2]]}, {t, 0, T2}, PlotLabels →
   {Style[ToString[Subscript[OverBar["β"], 11], FormatType → StandardForm] <> "=2.99" ,
     FontSize → 20], Style[ToString[Subscript[OverBar["β"], 11],
       FormatType → StandardForm] <> "=5" , FontSize → 20]},
  TicksStyle → Directive[Black, 20], PlotRange → Automatic,
  PlotStyle → {Green, Red}, ImageSize → Large]
```

Out[357]=

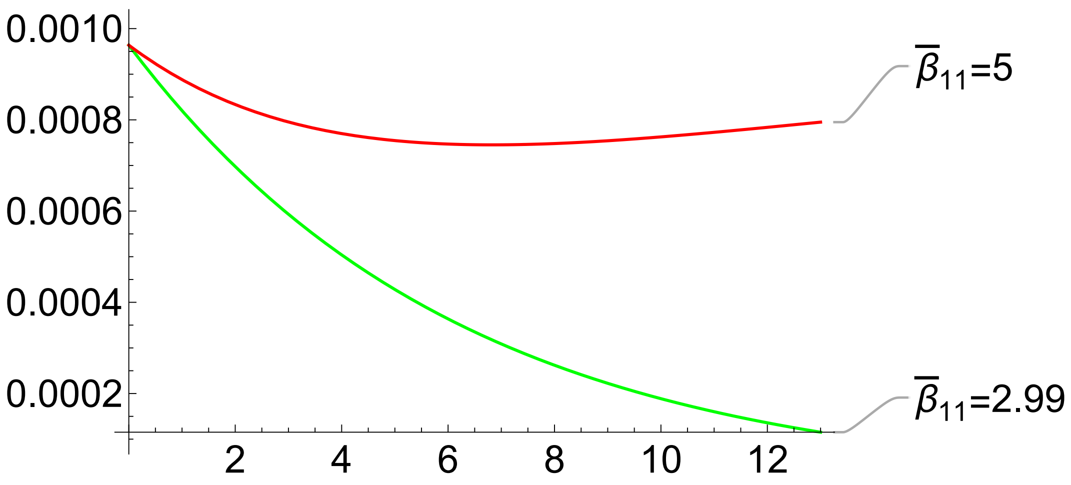
0.0010
0.0008
0.0006
0.0004
0.0002
2
4
6
8
10
12
$\overline{\beta}_{11}$=5
$\overline{\beta}_{11}$=2.99

## Phase Transition with varying two values of $\beta_{11}$ and $\overline{\beta}_{11}$ during Lock Down (Figure 6)

In[358]:=

```
F[a_, b_, c_, d_, x_, y_, para_] := Module[{u1 = a /. para /. bba11 → x /. bbb11 → y,
    u2 = b /. para /. bba11 → x /. bbb11 → y, v1 = c /. para /. bba11 → x /. bbb11 → y,
    v2 = d /. para /. bba11 → x /. bbb11 → y, bba11 = x, bbb11 = y}, NSolve[
     {((gg s1i - gg u1 + bbb11 s1i (-s1i + u1 + v1) + bbb12 s1i (-s2i + u2 + v2)) /. para) == 0,
      ((gg s2i - gg u2 + bbb21 s2i (-s1i + u1 + v1) + bbb22 s2i (-s2i + u2 + v2)) /. para) == 0},
     {s1i, s2i}] // Last];
para = {gg → 1, bbb22 → 1, bba22 → 2, bbb12 → 0.25, bbb21 → 0.25,
   bba12 → 0.5, bba21 → 0.5, tau → 5, n1 -> 0.2,
   n2 → 0.8, ia0 → 0, sa0 → 0.2 - 0, ib0 → 0.00003, sb0 → 0.8 - 0.00003};
BA = { { bba11 n1, bba12 n1}, {bba21 n2, bba22 n2}};
BB = { { bbb11 s1i, bbb12 s1i}, {bbb21 s2i, bbb22 s2i}};
I0 = {ia0, ib0};
S0 = {sa0, sb0};
{u1, u2} = (S0 - BA.Inverse[BA - gg IdentityMatrix[2]].
      ((MatrixExp[tau (BA - gg IdentityMatrix[2])]) - IdentityMatrix[2]).I0);
{v1, v2} = (MatrixExp[tau (BA - gg IdentityMatrix[2])].I0);
Plot3D[1 - {s1i + s2i} /. F[u1, u2, v1, v2, bba11, bbb11, para] // Total,
  {bba11, 0, 17}, {bbb11, 0.1, 15}, AxesLabel →
   {"β11,", ToString[Subscript[OverBar["β"], 11], FormatType → StandardForm]},
  ClippingStyle → None, ColorFunction →
   Function[{x, y, z}, If[z < 0.15, Hue[-z^(1/2) - 1/2 - 1/10], Hue[-0.15^(1/2) - 1/2 - 1/10]]], Mesh → 20]
```

Out[366]=

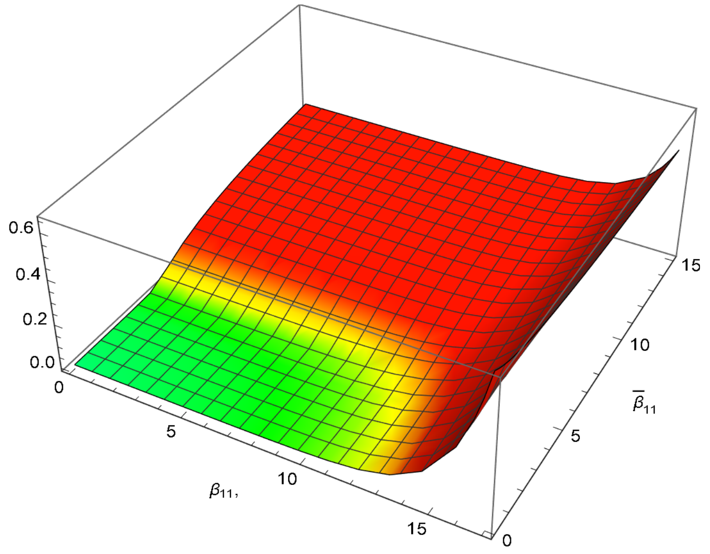


## Linear approximation during lockdown period for varying $\overline{\beta}_{11}$(Figure 5)

In[367]:=

```
gg = 1;
ss10 = 0.15;
```

```
ii10 = .0001;
ss20 = .7;
ii20 = .0001;
T = 15;
bb11 = 0;
bb22 = 1;
bb12 = 0.25;
bb21 = bb12;
v = 0.1;
SSS = NDSolve[{
    SS1'[t] == -bb11 SS1[t] × II1[t] - bb12 SS1[t] × II2[t],
    II1'[t] == bb11 SS1[t] × II1[t] + bb12 SS1[t] × II2[t] - gg II1[t],
    SS2'[t] == -bb21 SS2[t] × II1[t] - bb22 SS2[t] × II2[t],
    II2'[t] == bb21 SS2[t] × II1[t] + bb22 SS2[t] × II2[t] - gg II2[t],
    SS1[0] == ss10, II1[0] == ii10, SS2[0] == ss20, II2[0] == ii20},
   {SS1[t], II1[t], SS2[t], II2[t]}, {t, 0, T}, Method → "ExplicitRungeKutta"];
SSSL = NDSolve[{
    SS1'[t] == -bb11 ss10 II1[t] - bb12 ss10 II2[t],
    II1'[t] == bb11 ss10 II1[t] + bb12 ss10 II2[t] - gg II1[t],
    SS2'[t] == -bb21 ss20 II1[t] - bb22 ss20 II2[t],
    II2'[t] == bb21 ss20 II1[t] + bb22 ss20 II2[t] - gg II2[t],
    SS1[0] == ss10, II1[0] == ii10, SS2[0] == ss20, II2[0] == ii20},
   {SS1[t], II1[t], SS2[t], II2[t]}, {t, 0, T}, Method → "ExplicitRungeKutta"];
bb11 = 3;
SSS33 = NDSolve[{
    SS1'[t] == -bb11 SS1[t] × II1[t] - bb12 SS1[t] × II2[t],
    II1'[t] == bb11 SS1[t] × II1[t] + bb12 SS1[t] × II2[t] - gg II1[t],
    SS2'[t] == -bb21 SS2[t] × II1[t] - bb22 SS2[t] × II2[t],
    II2'[t] == bb21 SS2[t] × II1[t] + bb22 SS2[t] × II2[t] - gg II2[t],
    SS1[0] == ss10, II1[0] == ii10, SS2[0] == ss20, II2[0] == ii20},
   {SS1[t], II1[t], SS2[t], II2[t]}, {t, 0, T}, Method → "ExplicitRungeKutta"];
SSSL3 = NDSolve[{
    SS1'[t] == -bb11 ss10 II1[t] - bb12 ss10 II2[t],
    II1'[t] == bb11 ss10 II1[t] + bb12 ss10 II2[t] - gg II1[t],
    SS2'[t] == -bb21 ss20 II1[t] - bb22 ss20 II2[t],
    II2'[t] == bb21 ss20 II1[t] + bb22 ss20 II2[t] - gg II2[t],
    SS1[0] == ss10, II1[0] == ii10, SS2[0] == ss20, II2[0] == ii20},
   {SS1[t], II1[t], SS2[t], II2[t]}, {t, 0, T}, Method → "ExplicitRungeKutta"];
bb11 = 5;
SSS5 = NDSolve[{
    SS1'[t] == -bb11 SS1[t] × II1[t] - bb12 SS1[t] × II2[t],
    II1'[t] == bb11 SS1[t] × II1[t] + bb12 SS1[t] × II2[t] - gg II1[t],
    SS2'[t] == -bb21 SS2[t] × II1[t] - bb22 SS2[t] × II2[t],
    II2'[t] == bb21 SS2[t] × II1[t] + bb22 SS2[t] × II2[t] - gg II2[t],
    SS1[0] == ss10, II1[0] == ii10, SS2[0] == ss20, II2[0] == ii20},
   {SS1[t], II1[t], SS2[t], II2[t]}, {t, 0, T}, Method → "ExplicitRungeKutta"];
SSSL5 = NDSolve[{
    SS1'[t] == -bb11 ss10 II1[t] - bb12 ss10 II2[t],
    II1'[t] == bb11 ss10 II1[t] + bb12 ss10 II2[t] - gg II1[t],
    SS2'[t] == -bb21 ss20 II1[t] - bb22 ss20 II2[t],
    II2'[t] == bb21 ss20 II1[t] + bb22 ss20 II2[t] - gg II2[t],
    SS1[0] == ss10, II1[0] == ii10, SS2[0] == ss20, II2[0] == ii20},
   {SS1[t], II1[t], SS2[t], II2[t]}, {t, 0, T}, Method → "ExplicitRungeKutta"];

Plot[{SSS[[1, 4, 2]] + SSS[[1, 2, 2]], SSSL[[1, 4, 2]] + SSSL[[1, 2, 2]],
```

```
 SSS33[[1, 4, 2]] + SSS33[[1, 2, 2]], SSSL3[[1, 4, 2]] + SSSL3[[1, 2, 2]],
 SSS5[[1, 4, 2]] + SSS5[[1, 2, 2]], SSSL5[[1, 4, 2]] + SSSL5[[1, 2, 2]]},
{t, 0, 15}, PlotLabels → {Style["simulation" <>
    ToString[Subscript[OverTilde["β"], 11], FormatType → StandardForm] <> "=6, " <>
    ToString[Subscript[OverTilde["β"], 11], FormatType → StandardForm] <> "=0" ,
   FontSize → 20] , Style["linear app. " <>
    ToString[Subscript[OverTilde["β"], 11], FormatType → StandardForm] <> "=6, " <>
    ToString[Subscript[OverTilde["β"], 11], FormatType → StandardForm] <> "=0" ,
   FontSize → 20], Style["simulation" <> ToString[Subscript[OverTilde["β"], 11],
     FormatType → StandardForm] <> "=6, " <> ToString[Subscript[OverTilde["β"], 11],
     FormatType → StandardForm] <> "=3" , FontSize → 20], Style["linear app. " <>
    ToString[Subscript[OverTilde["β"], 11], FormatType → StandardForm] <> "=6, " <>
    ToString[Subscript[OverTilde["β"], 11], FormatType → StandardForm] <> "=3" ,
   FontSize → 20], Style["simulation" <>
    ToString[Subscript[OverTilde["β"], 11], FormatType → StandardForm] <> "=6, " <>
    ToString[Subscript[OverTilde["β"], 11], FormatType → StandardForm] <> "=5" ,
   FontSize → 20], Style["linear app. " <> ToString[Subscript[OverTilde["β"], 11],
     FormatType → StandardForm] <> "=6, " <> ToString[Subscript[OverTilde["β"], 11],
     FormatType → StandardForm] <> "=5" , FontSize → 20]},
Ticks → {Table[{i, i + 7}, {i, 0, 14}], Automatic},
AxesLabel →
 {Style["t", FontSize → 14], Style["I(t)", FontSize → 14]},
PlotRange → {0, 0.0002},
ImageSize → Large]
```

Out[386]=

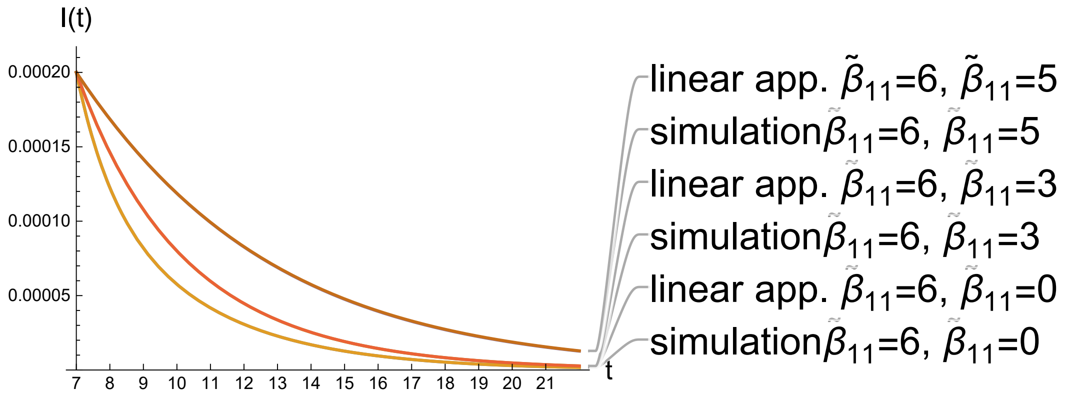

# VACCINATION PHASE

## Vaccination phase with school closed

In[387]:=
```
gg = 1;
ss10 = SSS0[[1, 1, 2]] /. t → T2;
ii10 = SSS0[[1, 2, 2]] /. t → T2;
ss20 = SSS0[[1, 3, 2]] /. t → T2;
ii20 = SSS0[[1, 4, 2]] /. t → T2;
T = 15;

bb22 = 2;
bb12 = 0.5;
bb21 = bb12;
v = 0.1;
bb11 = 0;
SV0 = NDSolve[{
     SS1'[t] == -bb11 SS1[t] × II1[t] - bb12 SS1[t] × II2[t],
     II1'[t] == bb11 SS1[t] × II1[t] + bb12 SS1[t] × II2[t] - gg II1[t],
     SS2'[t] == -bb21 SS2[t] × II1[t] - bb22 SS2[t] × II2[t] - v SS2[t],
     II2'[t] == bb21 SS2[t] × II1[t] + bb22 SS2[t] × II2[t] - gg II2[t],
     SS1[0] == ss10, II1[0] == ii10, SS2[0] == ss20, II2[0] == ii20},
    {SS1[t], II1[t], SS2[t], II2[t]}, {t, 0, T}, Method → "ExplicitRungeKutta"];
fig3 = Plot[{SV0[[1, 4, 2]] + SV0[[1, 2, 2]]}, {t, 0, T2},
  PlotLabels → {Style[ToString[Subscript[OverTilde["β"], 11],
       FormatType → StandardForm] <> "=0", FontSize → 20]},
  PlotLegends → Placed[{Style["Schools Closed", FontSize → 12]}, Center],
  PlotRange → {0, 0.0010}, PlotStyle → Cyan, ImageSize → Large]
```

Out[399]=

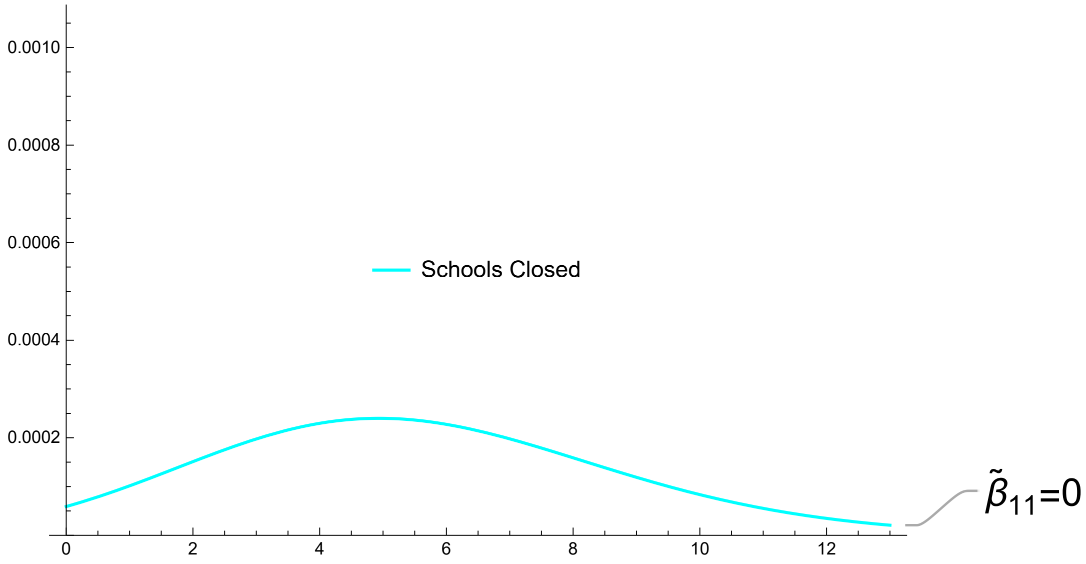

## Phase transition over vaccination phase

In[400]:=
```
gg = 1;
ss10 = SSS3[[1, 1, 2]] /. t → T2;
ii10 = SSS3[[1, 2, 2]] /. t → T2;
ss20 = SSS3[[1, 3, 2]] /. t → T2;
ii20 = SSS3[[1, 4, 2]] /. t → T2;
T = 15;

bb22 = 2;
bb12 = 0.5;
bb21 = bb12;
v = 0.1;
bb11 = 3;
SV3 = NDSolve[{
    SS1'[t] == -bb11 SS1[t] × II1[t] - bb12 SS1[t] × II2[t],
    II1'[t] == bb11 SS1[t] × II1[t] + bb12 SS1[t] × II2[t] - gg II1[t],
    SS2'[t] == -bb21 SS2[t] × II1[t] - bb22 SS2[t] × II2[t] - v SS2[t],
    II2'[t] == bb21 SS2[t] × II1[t] + bb22 SS2[t] × II2[t] - gg II2[t],
    SS1[0] == ss10, II1[0] == ii10, SS2[0] == ss20, II2[0] == ii20},
   {SS1[t], II1[t], SS2[t], II2[t]}, {t, 0, T}, Method → "ExplicitRungeKutta"];
bb11 = 5.02;
SV5 = NDSolve[{
    SS1'[t] == -bb11 SS1[t] × II1[t] - bb12 SS1[t] × II2[t],
    II1'[t] == bb11 SS1[t] × II1[t] + bb12 SS1[t] × II2[t] - gg II1[t],
    SS2'[t] == -bb21 SS2[t] × II1[t] - bb22 SS2[t] × II2[t] - v SS2[t],
    II2'[t] == bb21 SS2[t] × II1[t] + bb22 SS2[t] × II2[t] - gg II2[t],
    SS1[0] == ss10, II1[0] == ii10, SS2[0] == ss20, II2[0] == ii20},
   {SS1[t], II1[t], SS2[t], II2[t]}, {t, 0, T}, Method → "ExplicitRungeKutta"];
bb11 = 6;
SV6 = NDSolve[{
    SS1'[t] == -bb11 SS1[t] × II1[t] - bb12 SS1[t] × II2[t],
    II1'[t] == bb11 SS1[t] × II1[t] + bb12 SS1[t] × II2[t] - gg II1[t],
    SS2'[t] == -bb21 SS2[t] × II1[t] - bb22 SS2[t] × II2[t] - v SS2[t],
    II2'[t] == bb21 SS2[t] × II1[t] + bb22 SS2[t] × II2[t] - gg II2[t],
    SS1[0] == ss10, II1[0] == ii10, SS2[0] == ss20, II2[0] == ii20},
   {SS1[t], II1[t], SS2[t], II2[t]}, {t, 0, T}, Method → "ExplicitRungeKutta"];
fig33 = Plot[{SV3[[1, 4, 2]] + SV3[[1, 2, 2]], SV5[[1, 4, 2]] + SV5[[1, 2, 2]]
  , SV6[[1, 4, 2]] + SV6[[1, 2, 2]]}, {t, 0, T2}, PlotLabels →
   {Style[ToString[Subscript[OverTilde["β"], 11], FormatType → StandardForm] <> "=3",
     FontSize → 20], Style[ToString[Subscript[OverTilde["β"], 11],
       FormatType → StandardForm] <> "=5.02", FontSize → 20],
    Style[ToString[Subscript[OverTilde["β"], 11], FormatType → StandardForm] <> "=6",
     FontSize → 20]}, PlotLegends →
   Placed[{Style["Open Schools with Suitable Measures", FontSize → 12],
     Style["Critical Value", FontSize → 12], Style[
      "School Transmission Exceeding the Critical Value", FontSize → 12]}, Center],
  AxesLabel → {Style["t", FontSize → 20], Style["I(t)", FontSize → 20]},
  TicksStyle → Directive[Black, 20],
  PlotRange → Automatic,
  PlotStyle → {Green, Orange, Red}, ImageSize → Large]
```

In[417]:=

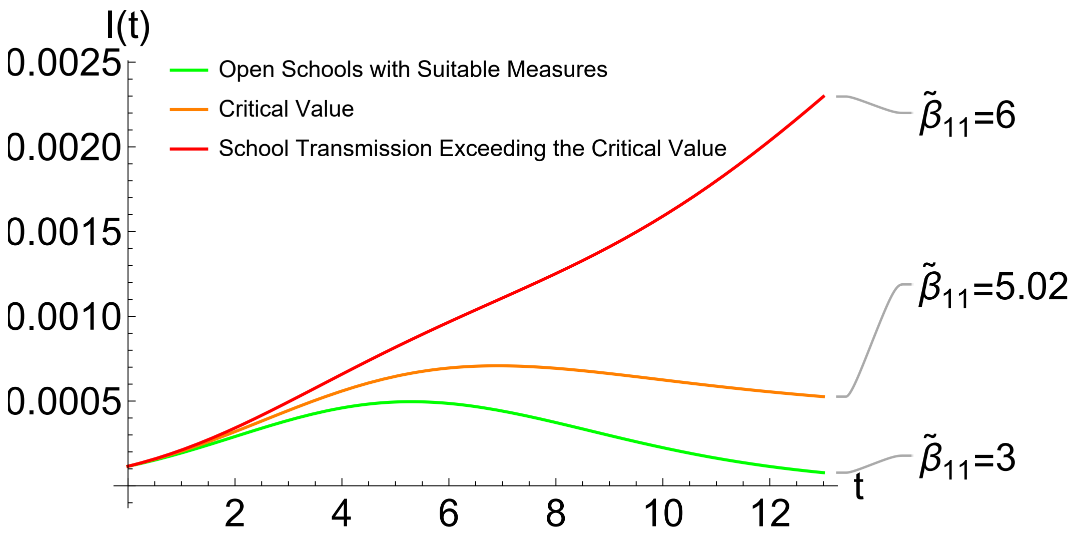


## Phase Transition with varying values of $\tilde{\beta}_{11}$ during Vaccination Period

In[418]:=

```
gg = 1;
ss10 = 0.2;
ii10 = 0;
ss20 = .79997;
ii20 = .00003;
T = 15;
bb11 = 10;
bb22 = 2;
bb12 = 0.5;
bb21 = bb12;
v = 0.1;
SSS = NDSolve[{
    SS1'[t] == -bb11 SS1[t] × II1[t] - bb12 SS1[t] × II2[t],
    II1'[t] == bb11 SS1[t] × II1[t] + bb12 SS1[t] × II2[t] - gg II1[t],
    SS2'[t] == -bb21 SS2[t] × II1[t] - bb22 SS2[t] × II2[t] - v SS2[t],
    II2'[t] == bb21 SS2[t] × II1[t] + bb22 SS2[t] × II2[t] - gg II2[t],
    SS1[0] == ss10, II1[0] == ii10, SS2[0] == ss20, II2[0] == ii20},
   {SS1[t], II1[t], SS2[t], II2[t]}, {t, 0, T}, Method → "ExplicitRungeKutta"];
bb11 = 0;
SSSC = NDSolve[{
    SS1'[t] == -bb11 SS1[t] × II1[t] - bb12 SS1[t] × II2[t],
    II1'[t] == bb11 SS1[t] × II1[t] + bb12 SS1[t] × II2[t] - gg II1[t],
    SS2'[t] == -bb21 SS2[t] × II1[t] - bb22 SS2[t] × II2[t] - v SS2[t],
    II2'[t] == bb21 SS2[t] × II1[t] + bb22 SS2[t] × II2[t] - gg II2[t],
    SS1[0] == ss10, II1[0] == ii10, SS2[0] == ss20, II2[0] == ii20},
   {SS1[t], II1[t], SS2[t], II2[t]}, {t, 0, T}, Method → "ExplicitRungeKutta"];
bb11 = 6;
bb22 = 2;
SSSL = NDSolve[{
    SS1'[t] == -bb11 SS1[t] × II1[t] - bb12 SS1[t] × II2[t],
    II1'[t] == bb11 SS1[t] × II1[t] + bb12 SS1[t] × II2[t] - gg II1[t],
    SS2'[t] == -bb21 SS2[t] × II1[t] - bb22 SS2[t] × II2[t] - v SS2[t],
    II2'[t] == bb21 SS2[t] × II1[t] + bb22 SS2[t] × II2[t] - gg II2[t],
    SS1[0] == ss10, II1[0] == ii10, SS2[0] == ss20, II2[0] == ii20},
   {SS1[t], II1[t], SS2[t], II2[t]}, {t, 0, T}, Method → "ExplicitRungeKutta"];
```

```
bb11 = 3;
bb22 = 2;
SSSL3 = NDSolve[{
    SS1'[t] == -bb11 SS1[t] × II1[t] - bb12 SS1[t] × II2[t],
    II1'[t] == bb11 SS1[t] × II1[t] + bb12 SS1[t] × II2[t] - gg II1[t],
    SS2'[t] == -bb21 SS2[t] × II1[t] - bb22 SS2[t] × II2[t] - v SS2[t],
    II2'[t] == bb21 SS2[t] × II1[t] + bb22 SS2[t] × II2[t] - gg II2[t],
    SS1[0] == ss10, II1[0] == ii10, SS2[0] == ss20, II2[0] == ii20},
   {SS1[t], II1[t], SS2[t], II2[t]}, {t, 0, T}, Method → "ExplicitRungeKutta"];
bb11 = 5;
bb22 = 2;
SSSL5 = NDSolve[{
    SS1'[t] == -bb11 SS1[t] × II1[t] - bb12 SS1[t] × II2[t],
    II1'[t] == bb11 SS1[t] × II1[t] + bb12 SS1[t] × II2[t] - gg II1[t],
    SS2'[t] == -bb21 SS2[t] × II1[t] - bb22 SS2[t] × II2[t] - v SS2[t],
    II2'[t] == bb21 SS2[t] × II1[t] + bb22 SS2[t] × II2[t] - gg II2[t],
    SS1[0] == ss10, II1[0] == ii10, SS2[0] == ss20, II2[0] == ii20},
   {SS1[t], II1[t], SS2[t], II2[t]}, {t, 0, T}, Method → "ExplicitRungeKutta"];

Plot[{SSSL[[1, 4, 2]] + SSSL[[1, 2, 2]],
  SSSL5[[1, 4, 2]] + SSSL5[[1, 2, 2]], SSSL3[[1, 4, 2]] + SSSL3[[1, 2, 2]]
  , SSSC[[1, 4, 2]] + SSSC[[1, 2, 2]]}, {t, 0, 15}, PlotLabels →
  {Style[ToString[Subscript[OverTilde["β"], 11], FormatType → StandardForm] <>
     "=6, " <> ToString[Subscript[OverTilde["β"], 11],
      FormatType → StandardForm] <> "=2" , FontSize → 20],
   Style[ToString[Subscript[OverTilde["β"], 11], FormatType → StandardForm] <>
     "=5, " <> ToString[Subscript[OverTilde["β"], 11],
      FormatType → StandardForm] <> "=2" , FontSize → 20],
   Style[ToString[Subscript[OverTilde["β"], 11], FormatType → StandardForm] <>
     "=3, " <> ToString[Subscript[OverTilde["β"], 11],
      FormatType → StandardForm] <> "=2" , FontSize → 20],
   Style[ToString[Subscript[OverTilde["β"], 11], FormatType → StandardForm] <>
     "=0, " <> ToString[Subscript[OverTilde["β"], 11],
      FormatType → StandardForm] <> "=2" , FontSize → 20]},
 AxesLabel → {Style["t", FontSize → 20], Style["I(t)", FontSize → 20]},
 PlotRange → {0, 0.0010},
 PlotStyle → {Red, Orange, Green, Cyan}, PlotLegends →
  Placed[{Style["School Transmission Exceeding the Critical Value", FontSize → 12],
    Style["Critical Value", FontSize → 12],
    Style["Open Schools with Suitable Measures", FontSize → 12],
    Style["Schools Closed", FontSize → 12]}, Center], ImageSize → Large]
```

In[442]:=

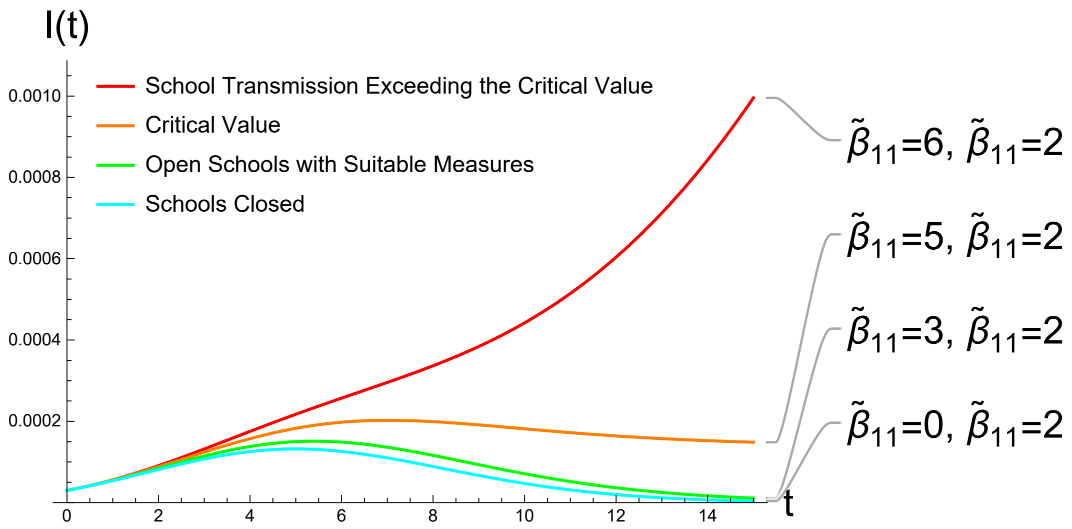
I(t)
School Transmission Exceeding the Critical Value
Critical Value
Open Schools with Suitable Measures
Schools Closed
0.0010
0.0008
0.0006
0.0004
0.0002
0
2
4
6
8
10
12
14
t
$\tilde{\beta}_{11}$=6, $\tilde{\beta}_{11}$=2
$\tilde{\beta}_{11}$=5, $\tilde{\beta}_{11}$=2
$\tilde{\beta}_{11}$=3, $\tilde{\beta}_{11}$=2
$\tilde{\beta}_{11}$=0, $\tilde{\beta}_{11}$=2

## Linear approximation with during vaccination period for varying $\tilde{\beta}_{11}$ (Figure 7)

In[443]:=

```
gg = 1;
ss10 = 0.2;
ii10 = 0;
ss20 = .79997;
ii20 = .00003;
T = 15;
bb12 = 0.5;
bb21 = bb12;
v = 0.1;
bb11 = 3;
bb22 = 2;
SSSL = NDSolve[{
    SS1'[t] == -bb11 SS1[t] × II1[t] - bb12 SS1[t] × II2[t],
    II1'[t] == bb11 SS1[t] × II1[t] + bb12 SS1[t] × II2[t] - gg II1[t],
    SS2'[t] == -bb21 SS2[t] × II1[t] - bb22 SS2[t] × II2[t] - v SS2[t],
    II2'[t] == bb21 SS2[t] × II1[t] + bb22 SS2[t] × II2[t] - gg II2[t],
    SS1[0] == ss10, II1[0] == ii10, SS2[0] == ss20, II2[0] == ii20},
   {SS1[t], II1[t], SS2[t], II2[t]}, {t, 0, T}, Method → "ExplicitRungeKutta"];

Equ = {II1'[t] == beta11 s10 II1[t] + beta12 s10 II2[t] - II1[t],
    II2'[t] == beta21 s20 E^(-vv t) II1[t] + beta22 s20 E^(-vv t) II2[t] - II2[t]} /.
   {gg → 1, beta11 → 3, beta22 → 2, beta12 → 0.5, beta21 → 0.5,
    tau → 2, ia0 → 0, s10 → 0.2, ib0 → 0.00003, s20 → 0.8 - 0.00003, vv → 0.1};

Inf1 = II1[t] /. NDSolve[{Equ[[1]], Equ[[2]],
     II1[0] == 0, II2[0] == 10^(-5)}, {II1[t], II2[t]}, {t, 0, 15}];
Inf2 = II2[t] /. NDSolve[{Equ[[1]], Equ[[2]],
     II1[0] == 0, II2[0] == 3 × 10^(-5)}, {II1[t], II2[t]}, {t, 0, 15}];

Plot[{SSSL[[1, 4, 2]], SSSL[[1, 2, 2]], Inf1, Inf2}, {t, 0, 12}, PlotLabels →
  {Style[ToString[Subscript[OverTilde["β"], 11], FormatType → StandardForm] <>
     "=3, " <> ToString[Subscript[OverTilde["β"], 11], FormatType → StandardForm] <>
     "=2" <> " - Infected outside", FontSize → 20],
   Style[ToString[Subscript[OverTilde["β"], 11], FormatType → StandardForm] <>
     "=3, " <> ToString[Subscript[OverTilde["β"], 11], FormatType → StandardForm] <>
     "=2" <> " - Infected in school", FontSize → 20],
   Style["linearization - Infected in school", FontSize → 20]
   , Style["linearization - Infected outside", FontSize → 20]},
 AxesLabel → {Style["t", FontSize → 20], Style["I(t)", FontSize → 20]},
 PlotRange → {0, 0.0002}, ImageSize → Large]
```

Out[458]=

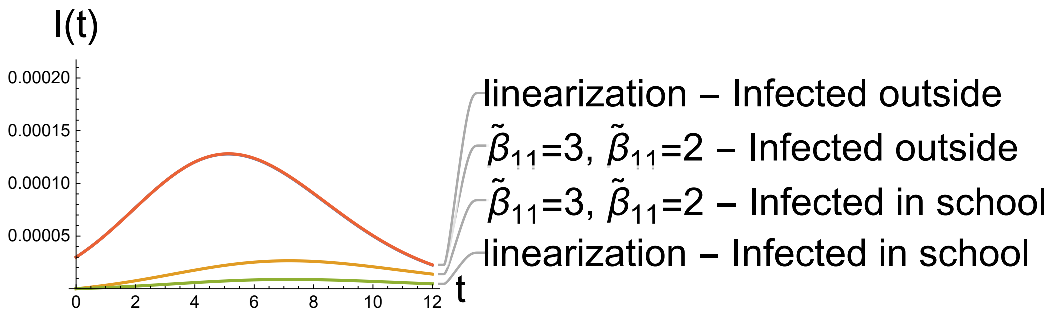


# Joint plot of phase transition in three phases (Figure 1)

In[467]:=

```
Show[fig1, fig2 /. l_Line :→ Translate[l, {T1, 0}],
 fig22 /. l_Line :→ Translate[l, {T1, 0}], fig3 /. l_Line :→ Translate[l, {T1 + T2, 0}],
 fig33 /. l_Line :→ Translate[l, {T1 + T2, 0}], PlotRange → All]
```

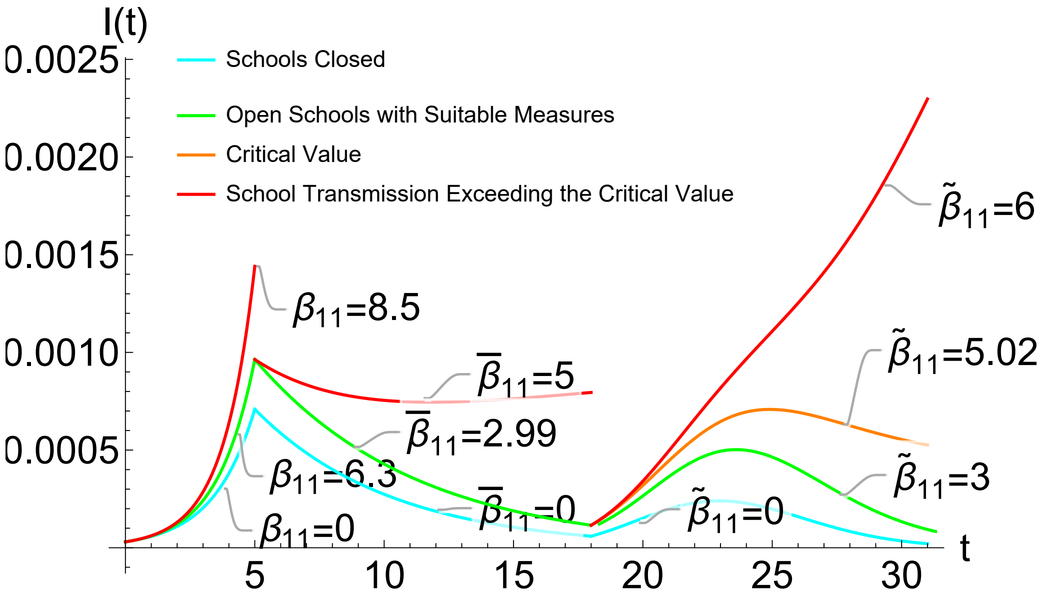

# Max Eigenvalue Transition (Figure 3,4)

In[460]:=
```
A = (a11 a12
     a21 a22) /. {a22 → 8, a12 → 0.5, a21 -> 0.5}
Eigenvalues[A] // Sort // Last
func[a11_] := 1/2 (8 + a11 + Sqrt[65.` - 16.` a11 + 1.` a11^2])
func[a]
ga = Plot[func'[a11], {a11, 0, 20}, PlotRange → {0, 1},
  AxesLabel → {Style["a11", FontSize → 20], Style["λ'max(a11)", FontSize → 20]}]
gb = Plot[func[a11], {a11, 0, 20}, PlotRange → Automatic,
  AxesLabel → {Style["a11", FontSize → 20], Style["λmax(a11)", FontSize → 20]}]
AA = {{a11, a12}, {a21, a22}}
```

Out[460]= {{a11, 0.5}, {0.5, 8}}

Out[461]= $\frac{1}{2}\left(8 + a11 + \sqrt{65. - 16.\, a11 + 1.\, a11^2}\right)$

Out[463]= $\frac{1}{2}\left(8 + a + \sqrt{65. - 16.\, a + 1.\, a^2}\right)$

Out[464]=
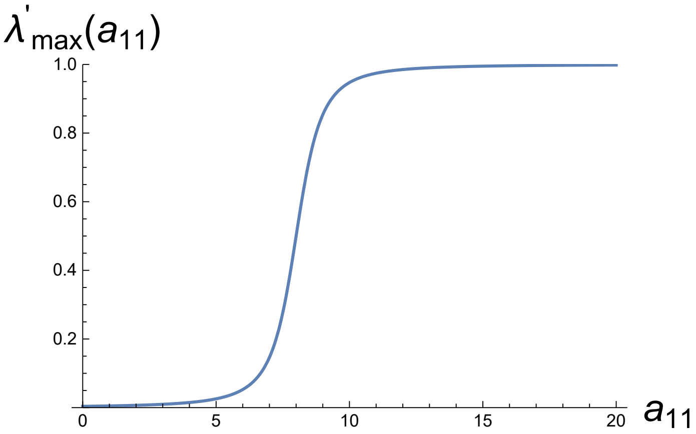


Out[465]=
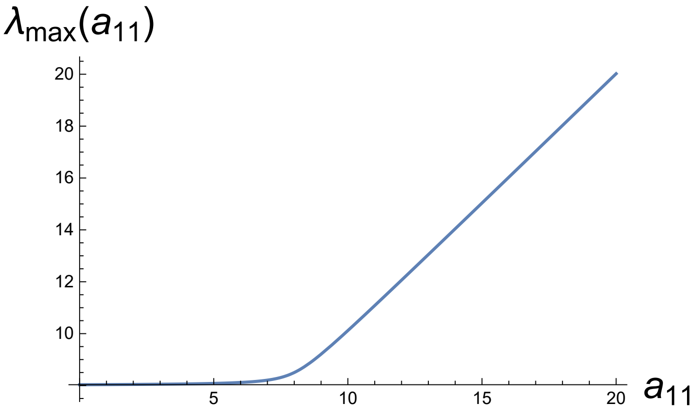


Out[466]= {{a11, a12}, {a21, a22}}
