# Supplementary material for: A new threshold reveals the uncertainty about the effect of school opening on diffusion of Covid-19
Source: arXiv:2104.04136 source file (2021-04-12)
Supplement: Supplementary file 3 [file MathStudySchoolOpening-OnlineMaterial-Spiar_model.pdf]

# SPIAR MODEL

This Mathematica file contains the simulations for a more elaborate model than SIR. We introduce the compartments of Susceptible S_i (not subjected to any virus transmission), Presymptomatic P_i (infected in incubation period), Asymptomatic A_i (infected not showing symptoms after incubation), Infected I_i and Recovered R_i for i=1,2 corresponding to the two subpopulations.

We consider the daily active cases, i.e., P+I+A := P_1+I_1+A_1+P_2+I_2+A_2, for three different scenarios (outbreak, lockdown, and vaccination), showing that phase transitions appear.

---

## FIRST SCENARIO: OUTBREAK PHASE

In[∘]:=
```
b11 = 0;
b12 = 0.25;
b21 = 0.25;
b22 = 2;
s = 0.9;
ξ = 0.3;
k = 1;
eps1 = 0.1;
eps2 = 0.3;
gamma = 1;


IP = 0.0001;

S10 = 0.16 * (1 - 2 * IP);
P10 =  0.16 * IP;
I10 = 0.16 * IP;
A10 = 0.0;
R10 = 0.0;
S20 = 0.84 * (1 - 2 * IP);
P20 = 0.84 * IP;
I20 = 0.84 * IP;
A20 = 0;
R20 = 0;

T = 5;

BETA0 = b11;
SPIAR = NDSolve[{
     S1'[t] == -b11 S1[t] (P1[t] + s A1[t]) - b12 S1[t] (ξ I2[t] + P2[t] + A2[t]),
     P1'[t] == b11 S1[t] (P1[t] + s A1[t]) + b12 S1[t] (ξ I2[t] + P2[t] + A2[t]) - k P1[t],
     I1'[t] == eps1 * k * P1[t] - gamma * I1[t],
     A1'[t] == (1 - eps1) * k * P1[t] - gamma * A1[t],
     R1'[t] == gamma * (A1[t] + I1[t]),
     S2'[t] ==
      -b21 S2[t] (ξ * I1[t] + P1[t] + A1[t]) - b22 S2[t] (ξ * I2[t] + P2[t] + A2[t]),
     P2'[t] == b21 S2[t] (ξ * I1[t] + P1[t] + A1[t]) +
       b22 S2[t] (ξ * I2[t] + P2[t] + A2[t]) - k * P2[t],
     I2'[t] == eps2 * k * P2[t] - gamma * I2[t],
     A2'[t] == (1 - eps2) * k * P2[t] - gamma * A2[t],
     R2'[t] == gamma * (A2[t] + I2[t]),
     S1[0] == S10, P1[0] == P10, I1[0] == I10, A1[0] == A10, R1[0] == R10,
     S2[0] == S20, P2[0] == P20, I2[0] == I20, A2[0] == A20, R2[0] == R20},
    {S1[t], P1[t], I1[t], A1[t], R1[t], S2[t], P2[t], I2[t], A2[t], R2[t]},
    {t, 0, T}, Method → "ExplicitRungeKutta"];
```

In[∘]:=

In[∘]:=
```
b11 = 8;
BETA1 = b11;
```

```
In[•]:= SPIAR1 = NDSolve[{
         S1'[t] == -b11 S1[t] (P1[t] + s A1[t]) - b12 S1[t] (ξ I2[t] + P2[t] + A2[t]),
         P1'[t] == b11 S1[t] (P1[t] + s A1[t]) + b12 S1[t] (ξ I2[t] + P2[t] + A2[t]) - k P1[t],
         I1'[t] == eps1 * k * P1[t] - gamma * I1[t],
         A1'[t] == (1 - eps1) * k * P1[t] - gamma * A1[t],
         R1'[t] == gamma * (A1[t] + I1[t]),
         S2'[t] ==
          -b21 S2[t] (ξ * I1[t] + P1[t] + A1[t]) - b22 S2[t] (ξ * I2[t] + P2[t] + A2[t]),
         P2'[t] == b21 S2[t] (ξ * I1[t] + P1[t] + A1[t]) +
           b22 S2[t] (ξ * I2[t] + P2[t] + A2[t]) - k * P2[t],
         I2'[t] == eps2 * k * P2[t] - gamma * I2[t],
         A2'[t] == (1 - eps2) * k * P2[t] - gamma * A2[t],
         R2'[t] == gamma * (A2[t] + I2[t]),
         S1[0] == S10, P1[0] == P10, I1[0] == I10, A1[0] == A10, R1[0] == R10,
         S2[0] == S20, P2[0] == P20, I2[0] == I20, A2[0] == A20, R2[0] == R20},
        {S1[t], P1[t], I1[t], A1[t], R1[t], S2[t], P2[t], I2[t], A2[t], R2[t]},
        {t, 0, T}, Method → "ExplicitRungeKutta"];

In[•]:= b11 = 11;
        BETA2 = b11;
```

In[∘]:=
```
SPIAR2 = NDSolve[{
    S1'[t] == -b11 S1[t] (P1[t] + s A1[t]) - b12 S1[t] (ξ I2[t] + P2[t] + A2[t]),
    P1'[t] == b11 S1[t] (P1[t] + s A1[t]) + b12 S1[t] (ξ I2[t] + P2[t] + A2[t]) - k P1[t],
    I1'[t] == eps1 * k * P1[t] - gamma * I1[t],
    A1'[t] == (1 - eps1) * k * P1[t] - gamma * A1[t],
    R1'[t] == gamma * (A1[t] + I1[t]),
    S2'[t] ==
     -b21 S2[t] (ξ * I1[t] + P1[t] + A1[t]) - b22 S2[t] (ξ * I2[t] + P2[t] + A2[t]),
    P2'[t] == b21 S2[t] (ξ * I1[t] + P1[t] + A1[t]) +
      b22 S2[t] (ξ * I2[t] + P2[t] + A2[t]) - k * P2[t],
    I2'[t] == eps2 * k * P2[t] - gamma * I2[t],
    A2'[t] == (1 - eps2) * k * P2[t] - gamma * A2[t],
    R2'[t] == gamma * (A2[t] + I2[t]),
    S1[0] == S10, P1[0] == P10, I1[0] == I10, A1[0] == A10, R1[0] == R10,
    S2[0] == S20, P2[0] == P20, I2[0] == I20, A2[0] == A20, R2[0] == R20},
   {S1[t], P1[t], I1[t], A1[t], R1[t], S2[t], P2[t], I2[t], A2[t], R2[t]},
   {t, 0, T}, Method → "ExplicitRungeKutta"];

Fig1 = Plot[{SPIAR[[1, 2, 2]] + SPIAR[[1, 3, 2]] +
    SPIAR[[1, 4, 2]] + SPIAR[[1, 7, 2]] + SPIAR[[1, 8, 2]] + SPIAR[[1, 9, 2]],
   SPIAR1[[1, 2, 2]] + SPIAR1[[1, 3, 2]] + SPIAR1[[1, 4, 2]] + SPIAR1[[1, 7, 2]] +
    SPIAR1[[1, 8, 2]] + SPIAR1[[1, 9, 2]], SPIAR2[[1, 2, 2]] + SPIAR2[[1, 3, 2]] +
    SPIAR2[[1, 4, 2]] + SPIAR2[[1, 7, 2]] + SPIAR2[[1, 8, 2]] + SPIAR2[[1, 9, 2]]},
  {t, 0, T}, PlotLabels → {Style[Subscript["β", 11] == BETA0, FontSize → 20],
    Style[Subscript["β", 11] == BETA1, FontSize → 20],
    Style[Subscript["β", 11] == BETA2, FontSize → 20]},
  AxesLabel → {Style["t", FontSize → 20], Style["P(t)+I(t)+A(t)", FontSize → 20]},
  PlotRange → {0, 0.12}, TicksStyle → Directive[Black, 20],
  PlotStyle → {Cyan, Green, Red}, ImageSize → Large]
```

Out[∘]=
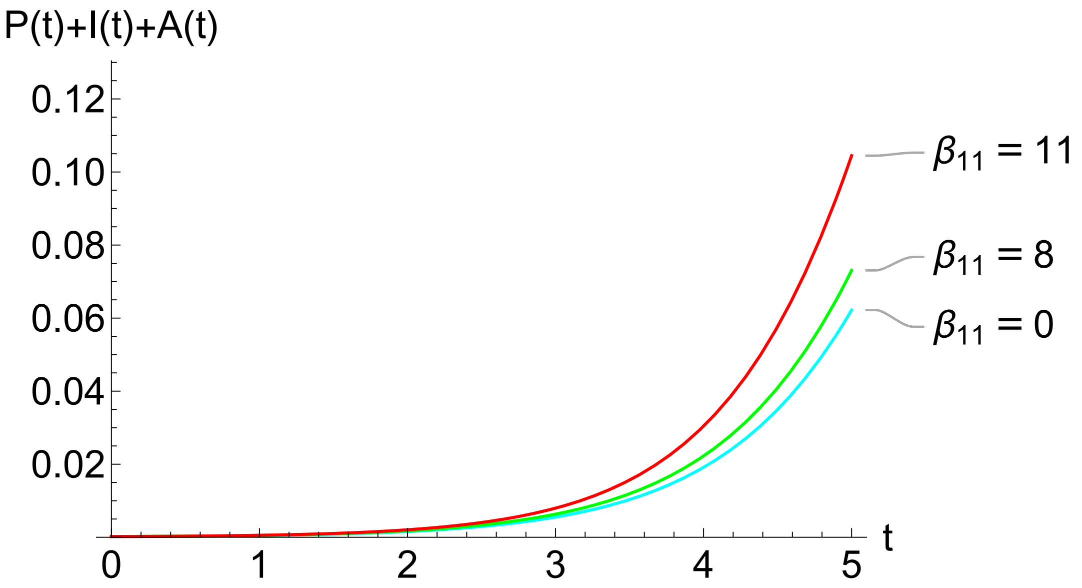


# SECOND SCENARIO: LOCKDOWN PHASE

In[∘]:=
```
Tf = 15;
```

```
T1 = T;
b11 = 0;
b12 = 0.1;
b21 = 0.1;
b22 = 0.5;

S10 = SPIAR[[1, 1, 2]] /. t → T1;
P10 = SPIAR[[1, 2, 2]] /. t → T1;
I10 = SPIAR[[1, 3, 2]] /. t → T1;
A10 = SPIAR[[1, 4, 2]] /. t → T1;
R10 = SPIAR[[1, 5, 2]] /. t → T1;
S20 = SPIAR[[1, 6, 2]] /. t → T1;
P20 = SPIAR[[1, 7, 2]] /. t → T1;
I20 = SPIAR[[1, 8, 2]] /. t → T1;
A20 = SPIAR[[1, 9, 2]] /. t → T1;
R20 = SPIAR[[1, 10, 2]] /. t → T1;

BETA0 = b11;
SPIARlock = NDSolve[{
    S1'[t] == -b11 S1[t] (P1[t] + s A1[t]) - b12 S1[t] (ξ I2[t] + P2[t] + A2[t]),
    P1'[t] == b11 S1[t] (P1[t] + s A1[t]) + b12 S1[t] (ξ I2[t] + P2[t] + A2[t]) - k P1[t],
    I1'[t] == eps1 * k * P1[t] - gamma * I1[t],
    A1'[t] == (1 - eps1) * k * P1[t] - gamma * A1[t],
    R1'[t] == gamma * (A1[t] + I1[t]),
    S2'[t] ==
     -b21 S2[t] (ξ * I1[t] + P1[t] + A1[t]) - b22 S2[t] (ξ * I2[t] + P2[t] + A2[t]),
    P2'[t] == b21 S2[t] (ξ * I1[t] + P1[t] + A1[t]) +
      b22 S2[t] (ξ * I2[t] + P2[t] + A2[t]) - k * P2[t],
    I2'[t] == eps2 * k * P2[t] - gamma * I2[t],
    A2'[t] == (1 - eps2) * k * P2[t] - gamma * A2[t],
    R2'[t] == gamma * (A2[t] + I2[t]),
    S1[0] == S10, P1[0] == P10, I1[0] == I10, A1[0] == A10, R1[0] == R10,
    S2[0] == S20, P2[0] == P20, I2[0] == I20, A2[0] == A20, R2[0] == R20},
   {S1[t], P1[t], I1[t], A1[t], R1[t], S2[t], P2[t], I2[t], A2[t], R2[t]},
   {t, 0, Tf}, Method → "ExplicitRungeKutta"];


S10 = SPIAR1[[1, 1, 2]] /. t → T1;
P10 = SPIAR1[[1, 2, 2]] /. t → T1;
I10 = SPIAR1[[1, 3, 2]] /. t → T1;
A10 = SPIAR1[[1, 4, 2]] /. t → T1;
R10 = SPIAR1[[1, 5, 2]] /. t → T1;
S20 = SPIAR1[[1, 6, 2]] /. t → T1;
P20 = SPIAR1[[1, 7, 2]] /. t → T1;
I20 = SPIAR1[[1, 8, 2]] /. t → T1;
A20 = SPIAR1[[1, 9, 2]] /. t → T1;
R20 = SPIAR1[[1, 10, 2]] /. t → T1;

b11 = 2;
BETA1 = b11;
SPIAR1lock = NDSolve[{
    S1'[t] == -b11 S1[t] (P1[t] + s A1[t]) - b12 S1[t] (ξ I2[t] + P2[t] + A2[t]),
    P1'[t] == b11 S1[t] (P1[t] + s A1[t]) + b12 S1[t] (ξ I2[t] + P2[t] + A2[t]) - k P1[t],
    I1'[t] == eps1 * k * P1[t] - gamma * I1[t],
    A1'[t] == (1 - eps1) * k * P1[t] - gamma * A1[t],
```

```
     R1'[t] == gamma * (A1[t] + I1[t]),
     S2'[t] ==
      -b21 S2[t] (ξ * I1[t] + P1[t] + A1[t]) - b22 S2[t] (ξ * I2[t] + P2[t] + A2[t]),
     P2'[t] == b21 S2[t] (ξ * I1[t] + P1[t] + A1[t]) +
       b22 S2[t] (ξ * I2[t] + P2[t] + A2[t]) - k * P2[t],
     I2'[t] == eps2 * k * P2[t] - gamma * I2[t],
     A2'[t] == (1 - eps2) * k * P2[t] - gamma * A2[t],
     R2'[t] == gamma * (A2[t] + I2[t]),
     S1[0] == S10, P1[0] == P10, I1[0] == I10, A1[0] == A10, R1[0] == R10,
     S2[0] == S20, P2[0] == P20, I2[0] == I20, A2[0] == A20, R2[0] == R20},
    {S1[t], P1[t], I1[t], A1[t], R1[t], S2[t], P2[t], I2[t], A2[t], R2[t]},
    {t, 0, Tf}, Method → "ExplicitRungeKutta"];

b11 = 6;
BETA2 = b11;
SPIAR2lock = NDSolve[{
     S1'[t] == -b11 S1[t] (P1[t] + s A1[t]) - b12 S1[t] (ξ I2[t] + P2[t] + A2[t]),
     P1'[t] == b11 S1[t] (P1[t] + s A1[t]) + b12 S1[t] (ξ I2[t] + P2[t] + A2[t]) - k P1[t],
     I1'[t] == eps1 * k * P1[t] - gamma * I1[t],
     A1'[t] == (1 - eps1) * k * P1[t] - gamma * A1[t],
     R1'[t] == gamma * (A1[t] + I1[t]),
     S2'[t] ==
      -b21 S2[t] (ξ * I1[t] + P1[t] + A1[t]) - b22 S2[t] (ξ * I2[t] + P2[t] + A2[t]),
     P2'[t] == b21 S2[t] (ξ * I1[t] + P1[t] + A1[t]) +
       b22 S2[t] (ξ * I2[t] + P2[t] + A2[t]) - k * P2[t],
     I2'[t] == eps2 * k * P2[t] - gamma * I2[t],
     A2'[t] == (1 - eps2) * k * P2[t] - gamma * A2[t],
     R2'[t] == gamma * (A2[t] + I2[t]),
     S1[0] == S10, P1[0] == P10, I1[0] == I10, A1[0] == A10, R1[0] == R10,
     S2[0] == S20, P2[0] == P20, I2[0] == I20, A2[0] == A20, R2[0] == R20},
    {S1[t], P1[t], I1[t], A1[t], R1[t], S2[t], P2[t], I2[t], A2[t], R2[t]},
    {t, 0, Tf}, Method → "ExplicitRungeKutta"];

Fig2 = Plot[{SPIARlock[[1, 2, 2]] + SPIARlock[[1, 3, 2]] + SPIARlock[[1, 4, 2]] +
     SPIARlock[[1, 7, 2]] + SPIARlock[[1, 8, 2]] + SPIARlock[[1, 9, 2]],
    SPIAR1lock[[1, 2, 2]] + SPIAR1lock[[1, 3, 2]] + SPIAR1lock[[1, 4, 2]] +
     SPIAR1lock[[1, 7, 2]] + SPIAR1lock[[1, 8, 2]] + SPIAR1lock[[1, 9, 2]],
    SPIAR2lock[[1, 2, 2]] + SPIAR2lock[[1, 3, 2]] + SPIAR2lock[[1, 4, 2]] +
     SPIAR2lock[[1, 7, 2]] + SPIAR2lock[[1, 8, 2]] + SPIAR2lock[[1, 9, 2]]}, {t, 0, Tf},
   PlotLabels → {Style[Subscript[OverBar["β"], 11] == BETA0, FontSize → 20],
     Style[Subscript[OverBar["β"], 11] == BETA1, FontSize → 20],
     Style[Subscript[OverBar["β"], 11] == BETA2, FontSize → 20]},
   AxesLabel → {Style["t", FontSize → 20], Style["P(t)+I(t)+A(t)", FontSize → 20]},
   PlotRange → Automatic, TicksStyle → Directive[Black, 20],
   PlotStyle → {Cyan, Green, Red}, ImageSize → Large]
```

Out[ ]=

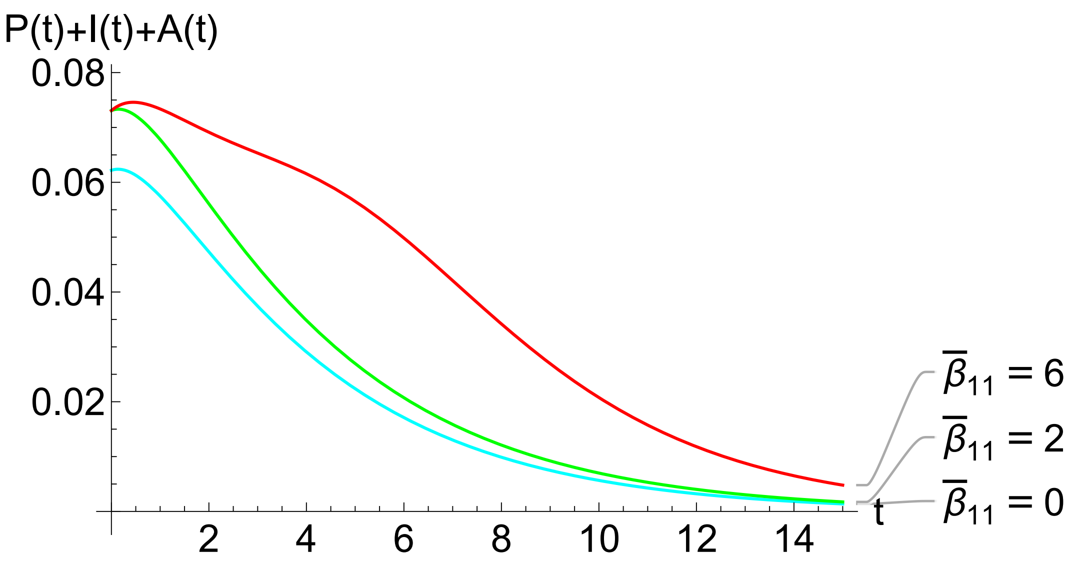
P(t)+I(t)+A(t)
0.08
0.06
0.04
0.02
2
4
6
8
10
12
14
t
$\overline{\beta}_{11} = 6$
$\overline{\beta}_{11} = 2$
$\overline{\beta}_{11} = 0$

In[ ]:=

# THIRD SCENARIO: VACCINATION PHASE

In[ ]:=
```
T2 = Tf;
Tfa = 20;
b11 = 0;
b12 = 0.25;
b21 = 0.25;
b22 = 1.5;
v = 0.2;

S10 = SPIARlock[[1, 1, 2]] /. t → T2;
P10 = SPIARlock[[1, 2, 2]] /. t → T2;
I10 = SPIARlock[[1, 3, 2]] /. t → T2;
A10 = SPIARlock[[1, 4, 2]] /. t → T2;
R10 = SPIARlock[[1, 5, 2]] /. t → T2;
S20 = SPIARlock[[1, 6, 2]] /. t → T2;
P20 = SPIARlock[[1, 7, 2]] /. t → T2;
I20 = SPIARlock[[1, 8, 2]] /. t → T2;
A20 = SPIARlock[[1, 9, 2]] /. t → T2;
R20 = SPIARlock[[1, 10, 2]] /. t → T2;

BETA0 = b11;
SPIARvacc = NDSolve[{
    S1'[t] == -b11 S1[t] (P1[t] + s A1[t]) - b12 S1[t] (ξ I2[t] + P2[t] + A2[t]),
    P1'[t] == b11 S1[t] (P1[t] + s A1[t]) + b12 S1[t] (ξ I2[t] + P2[t] + A2[t]) - k P1[t],
    I1'[t] == eps1 * k * P1[t] - gamma * I1[t],
    A1'[t] == (1 - eps1) * k * P1[t] - gamma * A1[t],
    R1'[t] == gamma * (A1[t] + I1[t]),
    S2'[t] ==
     -b21 S2[t] (ξ * I1[t] + P1[t] + A1[t]) - b22 S2[t] (ξ * I2[t] + P2[t] + A2[t]) - v S1[t],
    P2'[t] == b21 S2[t] (ξ * I1[t] + P1[t] + A1[t]) +
      b22 S2[t] (ξ * I2[t] + P2[t] + A2[t]) - k * P2[t],
    I2'[t] == eps2 * k * P2[t] - gamma * I2[t],
    A2'[t] == (1 - eps2) * k * P2[t] - gamma * A2[t],
    R2'[t] == gamma * (A2[t] + I2[t]) + v S1[t],
    S1[0] == S10, P1[0] == P10, I1[0] == I10, A1[0] == A10, R1[0] == R10,
    S2[0] == S20, P2[0] == P20, I2[0] == I20, A2[0] == A20, R2[0] == R20},
   {S1[t], P1[t], I1[t], A1[t], R1[t], S2[t], P2[t], I2[t], A2[t], R2[t]},
   {t, 0, Tfa}, Method → "ExplicitRungeKutta"];
```

In[ ]:=
```
S10 = SPIAR1lock[[1, 1, 2]] /. t → T2;
P10 = SPIAR1lock[[1, 2, 2]] /. t → T2;
I10 = SPIAR1lock[[1, 3, 2]] /. t → T2;
A10 = SPIAR1lock[[1, 4, 2]] /. t → T2;
R10 = SPIAR1lock[[1, 5, 2]] /. t → T2;
S20 = SPIAR1lock[[1, 6, 2]] /. t → T2;
P20 = SPIAR1lock[[1, 7, 2]] /. t → T2;
I20 = SPIAR1lock[[1, 8, 2]] /. t → T2;
A20 = SPIAR1lock[[1, 9, 2]] /. t → T2;
R20 = SPIAR1lock[[1, 10, 2]] /. t → T2;

b11 = 3;
BETA1 = b11;
SPIAR1vacc = NDSolve[{
```

```
    S1'[t] == -b11 S1[t] (P1[t] + s A1[t]) - b12 S1[t] (ξ I2[t] + P2[t] + A2[t]),
    P1'[t] == b11 S1[t] (P1[t] + s A1[t]) + b12 S1[t] (ξ I2[t] + P2[t] + A2[t]) - k P1[t],
    I1'[t] == eps1 * k * P1[t] - gamma * I1[t],
    A1'[t] == (1 - eps1) * k * P1[t] - gamma * A1[t],
    R1'[t] == gamma * (A1[t] + I1[t]),
    S2'[t] ==
     -b21 S2[t] (ξ * I1[t] + P1[t] + A1[t]) - b22 S2[t] (ξ * I2[t] + P2[t] + A2[t]) - v S1[t],
    P2'[t] == b21 S2[t] (ξ * I1[t] + P1[t] + A1[t]) +
      b22 S2[t] (ξ * I2[t] + P2[t] + A2[t]) - k * P2[t],
    I2'[t] == eps2 * k * P2[t] - gamma * I2[t],
    A2'[t] == (1 - eps2) * k * P2[t] - gamma * A2[t],
    R2'[t] == gamma * (A2[t] + I2[t]) + v S1[t],
    S1[0] == S10, P1[0] == P10, I1[0] == I10, A1[0] == A10, R1[0] == R10,
    S2[0] == S20, P2[0] == P20, I2[0] == I20, A2[0] == A20, R2[0] == R20},
   {S1[t], P1[t], I1[t], A1[t], R1[t], S2[t], P2[t], I2[t], A2[t], R2[t]},
   {t, 0, Tfa}, Method → "ExplicitRungeKutta"];

b11 = 5;
BETA2 = b11;
SPIAR2vacc = NDSolve[{
    S1'[t] == -b11 S1[t] (P1[t] + s A1[t]) - b12 S1[t] (ξ I2[t] + P2[t] + A2[t]),
    P1'[t] == b11 S1[t] (P1[t] + s A1[t]) + b12 S1[t] (ξ I2[t] + P2[t] + A2[t]) - k P1[t],
    I1'[t] == eps1 * k * P1[t] - gamma * I1[t],
    A1'[t] == (1 - eps1) * k * P1[t] - gamma * A1[t],
    R1'[t] == gamma * (A1[t] + I1[t]),
    S2'[t] ==
     -b21 S2[t] (ξ * I1[t] + P1[t] + A1[t]) - b22 S2[t] (ξ * I2[t] + P2[t] + A2[t]) - v S1[t],
    P2'[t] == b21 S2[t] (ξ * I1[t] + P1[t] + A1[t]) +
      b22 S2[t] (ξ * I2[t] + P2[t] + A2[t]) - k * P2[t],
    I2'[t] == eps2 * k * P2[t] - gamma * I2[t],
    A2'[t] == (1 - eps2) * k * P2[t] - gamma * A2[t],
    R2'[t] == gamma * (A2[t] + I2[t]) + v S1[t],
    S1[0] == S10, P1[0] == P10, I1[0] == I10, A1[0] == A10, R1[0] == R10,
    S2[0] == S20, P2[0] == P20, I2[0] == I20, A2[0] == A20, R2[0] == R20},
   {S1[t], P1[t], I1[t], A1[t], R1[t], S2[t], P2[t], I2[t], A2[t], R2[t]},
   {t, 0, Tfa}, Method → "ExplicitRungeKutta"];

b11 = 8;
BETA3 = b11;
SPIAR3vacc = NDSolve[{
    S1'[t] == -b11 S1[t] (P1[t] + s A1[t]) - b12 S1[t] (ξ I2[t] + P2[t] + A2[t]),
    P1'[t] == b11 S1[t] (P1[t] + s A1[t]) + b12 S1[t] (ξ I2[t] + P2[t] + A2[t]) - k P1[t],
    I1'[t] == eps1 * k * P1[t] - gamma * I1[t],
    A1'[t] == (1 - eps1) * k * P1[t] - gamma * A1[t],
    R1'[t] == gamma * (A1[t] + I1[t]),
    S2'[t] ==
     -b21 S2[t] (ξ * I1[t] + P1[t] + A1[t]) - b22 S2[t] (ξ * I2[t] + P2[t] + A2[t]) - v S1[t],
    P2'[t] == b21 S2[t] (ξ * I1[t] + P1[t] + A1[t]) +
      b22 S2[t] (ξ * I2[t] + P2[t] + A2[t]) - k * P2[t],
    I2'[t] == eps2 * k * P2[t] - gamma * I2[t],
    A2'[t] == (1 - eps2) * k * P2[t] - gamma * A2[t],
    R2'[t] == gamma * (A2[t] + I2[t]) + v S1[t],
    S1[0] == S10, P1[0] == P10, I1[0] == I10, A1[0] == A10, R1[0] == R10,
    S2[0] == S20, P2[0] == P20, I2[0] == I20, A2[0] == A20, R2[0] == R20},
   {S1[t], P1[t], I1[t], A1[t], R1[t], S2[t], P2[t], I2[t], A2[t], R2[t]},
```

```
    {t, 0, Tfa}, Method → "ExplicitRungeKutta"];

Fig3 = Plot[{SPIARvacc[[1, 2, 2]] + SPIARvacc[[1, 3, 2]] + SPIARvacc[[1, 4, 2]] +
     SPIARvacc[[1, 7, 2]] + SPIARvacc[[1, 8, 2]] + SPIARvacc[[1, 9, 2]],
    SPIAR1vacc[[1, 2, 2]] + SPIAR1vacc[[1, 3, 2]] + SPIAR1vacc[[1, 4, 2]] +
     SPIAR1vacc[[1, 7, 2]] + SPIAR1vacc[[1, 8, 2]] + SPIAR1vacc[[1, 9, 2]],
    SPIAR2vacc[[1, 2, 2]] + SPIAR2vacc[[1, 3, 2]] + SPIAR2vacc[[1, 4, 2]] +
     SPIAR2vacc[[1, 7, 2]] + SPIAR2vacc[[1, 8, 2]] + SPIAR2vacc[[1, 9, 2]],
    SPIAR3vacc[[1, 2, 2]] + SPIAR3vacc[[1, 3, 2]] + SPIAR3vacc[[1, 4, 2]] +
     SPIAR3vacc[[1, 7, 2]] + SPIAR3vacc[[1, 8, 2]] + SPIAR3vacc[[1, 9, 2]]}, {t, 0, Tfa},
   PlotLabels → {Style[Subscript[OverTilde["β"], 11] == BETA0, FontSize → 20],
     Style[Subscript[OverTilde["β"], 11] == BETA1, FontSize → 20],
     Style[Subscript[OverTilde["β"], 11] == BETA2, FontSize → 20],
     Style[Subscript[OverTilde["β"], 11] == BETA3, FontSize → 20]},
   PlotLegends → Placed[{Style["Schools Closed", FontSize → 12],
      Style["Open Schools with Suitable Measures", FontSize → 12],
      Style["Critical Value", FontSize → 12],
      Style["School Transmission Exceeding the Critical Value", FontSize → 12]},
     Center],
   AxesLabel → {Style["t", FontSize → 20], Style["P(t)+I(t)+A(t)", FontSize → 20]},
   TicksStyle → Directive[Black, 20], PlotRange → Automatic,
   PlotStyle → {Cyan, Green, Orange, Red}, ImageSize → Large]
```

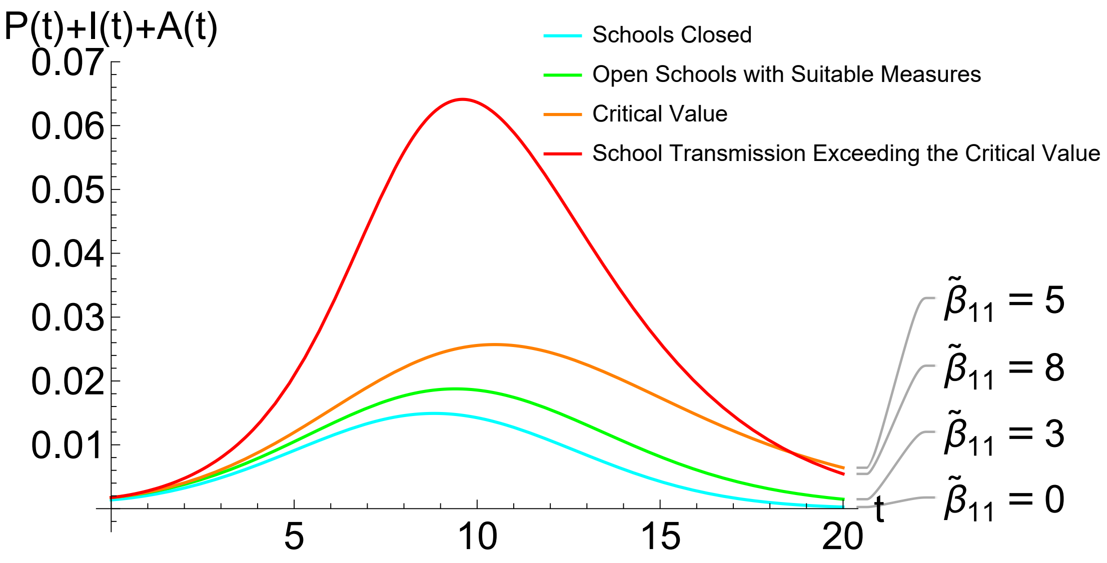


# CUMULATIVE PLOT: OUTBREAK + LOCKDOWN + VACCINATION (FIGURE 8 in the paper)

```
In[]:= Show[Fig1 /. l_Line :> Translate[l, {0, 0}], Fig2 /. l_Line :> Translate[l, {T1, 0}],
        Fig3 /. l_Line :> Translate[l, {Tfa, 0}], PlotRange → All]
```

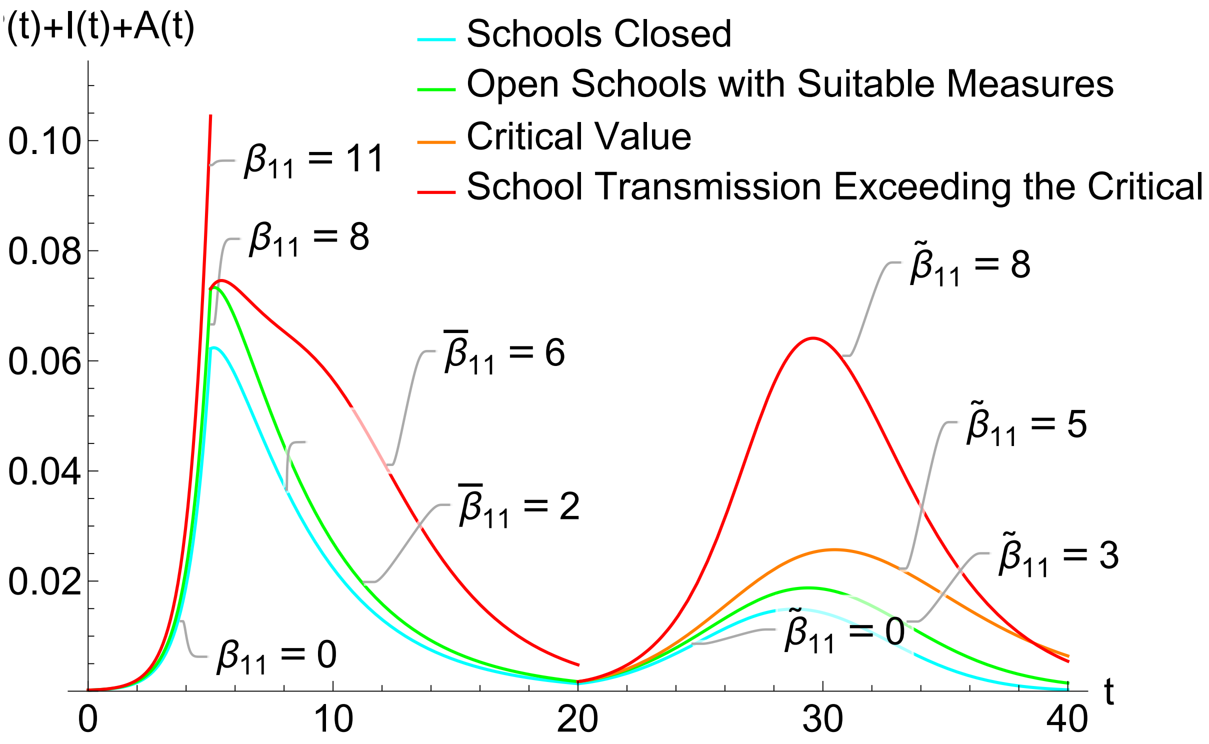
(t)+I(t)+A(t)
Schools Closed
Open Schools with Suitable Measures
Critical Value
School Transmission Exceeding the Critical
β11 = 11
β11 = 8
β̄11 = 6
β̄11 = 2
β11 = 0
β̃11 = 8
β̃11 = 5
β̃11 = 3
β̃11 = 0
0.10
0.08
0.06
0.04
0.02
0
10
20
30
40
t
